# Supplementary material for: Causal language jumps in clinical practice guidelines for diabetes management
Source: arXiv:2503.03557 ancillary file (2025-03-05)
Supplement: Supplementary file 1 [file supplementary_files.pdf]

---

# **Causal language jumps in clinical practice guidelines for diabetes management**

## **Supplementary data**

4 March 2025

---

---

### **File contents**

File S1 Guideline characteristics

File S2 Details of scales used for rating

File S3 Original study characteristics

File S4 Causal linking words in guidelines and original studies

---

# Contents

|                |                                                                        |           |
|----------------|------------------------------------------------------------------------|-----------|
| <b>File S1</b> | <b>Guideline characteristics</b>                                       | <b>3</b>  |
| S1.1           | Guideline and original study characteristics . . . . .                 | 3         |
| S1.2           | Word use characteristics in guideline statements and recommendations . | 5         |
| S1.3           | Original study sentence characteristics . . . . .                      | 6         |
| <b>File S2</b> | <b>Details of scales used for rating</b>                               | <b>9</b>  |
| S2.1           | Scale for causation strength . . . . .                                 | 9         |
| S2.2           | Scale for recommendation causation-dependence . . . . .                | 11        |
| S2.3           | Scale for target trial emulation components . . . . .                  | 13        |
| S2.4           | Examples for rating . . . . .                                          | 18        |
| <b>File S3</b> | <b>Original study characteristics</b>                                  | <b>21</b> |
| <b>File S4</b> | <b>Causal linking words in guidelines and original studies</b>         | <b>53</b> |
|                | <b>References cited in supplementary files</b>                         | <b>57</b> |



# **File S1**

## **Guideline characteristics**

### **S1.1 Guideline and original study characteristics**

Table S1.1: Guideline characteristics

| Title                                                                                              | Year | Association                               | Topic                                         | No. eligible sentences | No. eligible rec.'s | No. sampled sentences | No. sampled rec.'s |
|----------------------------------------------------------------------------------------------------|------|-------------------------------------------|-----------------------------------------------|------------------------|---------------------|-----------------------|--------------------|
| ADA Standards of Care in Diabetes—2024                                                             | 2023 | American Diabetes Association             | general diabetes care                         | 898                    | 94                  | 230                   | 70                 |
| - Section 3: Prevention or Delay of Diabetes and Associated Comorbidities [1]                      |      |                                           | prevention of DM and treatment of prediabetes | 93                     | 12                  | 17                    | 6                  |
| - Section 5: Facilitating Positive Health Behaviors and Well-being to Improve Health Outcomes [2]  |      |                                           | lifestyle management for diabetes             | 558                    | 49                  | 147                   | 42                 |
| - Section 8: Obesity and Weight Management for the Prevention and Treatment of Type 2 Diabetes [3] |      |                                           | treatment of obesity                          | 59                     | 13                  | 16                    | 10                 |
| - Section 10: Cardiovascular Disease and Risk Management [4]                                       |      |                                           | cardiovascular risk and diabetes              | 108                    | 10                  | 29                    | 7                  |
| - Section 13: Older Adults [5]                                                                     |      |                                           | diabetes in geriatric population              | 80                     | 10                  | 21                    | 5                  |
| 2023 ESC Guidelines for the management of cardiovascular disease in patients with diabetes [6]     | 2023 | European Society of Cardiology and others | cardiovascular risk and diabetes              | 131                    | 13                  | 30                    | 13                 |

Causal language jumps in guidelines

Table S1.1 (Continued)

| Title                                                         | Year | Association                       | Topic                            | No. eligible sentences | No. eligible rec.'s | No. sampled sentences | No. sampled rec.'s |
|---------------------------------------------------------------|------|-----------------------------------|----------------------------------|------------------------|---------------------|-----------------------|--------------------|
| Global guideline for Type 2 Diabetes                          | 2012 | International Diabetes Federation | general diabetes care            | 30                     | N/A                 | 9                     | N/A                |
| Managing older people with type 2 diabetes. Global guideline. | 2014 | International Diabetes Federation | diabetes in geriatric population | 116                    | N/A                 | 31                    | N/A                |

rec., recommendations.

## S1.2 Word use characteristics in guideline statements and recommendations

### S1.3 Original study sentence characteristics

Table S1.2: Characteristics for sentences from original studies

| Source                           | Character             | Length             | Top 5 candidate causal linking words (count of occurrence)              |
|----------------------------------|-----------------------|--------------------|-------------------------------------------------------------------------|
| Abstract conclusive sentences    | 173.0 (126.8 – 213.2) | 20.0 (15.8 – 25.3) | risk (27), improve (22), significant (21), associated (20), effect (17) |
| Abstract action recommendations  | 131.0 (98.0 – 182.0)  | 16.0 (12.0 – 21.5) | benefit (6), improve (6), effect (6), associated (3), risk (3)          |
| Main text conclusive sentences   | 160.0 (126.0 – 207.0) | 19.0 (15.0 – 24.3) | associated (25), significant (22), risk (19), improve (19), effect (18) |
| Main text action recommendations | 167.0 (129.0 – 248.0) | 20.0 (14.8 – 32.3) | prevent (12), risk (11), reduce (11), effect (10), improve (9)          |

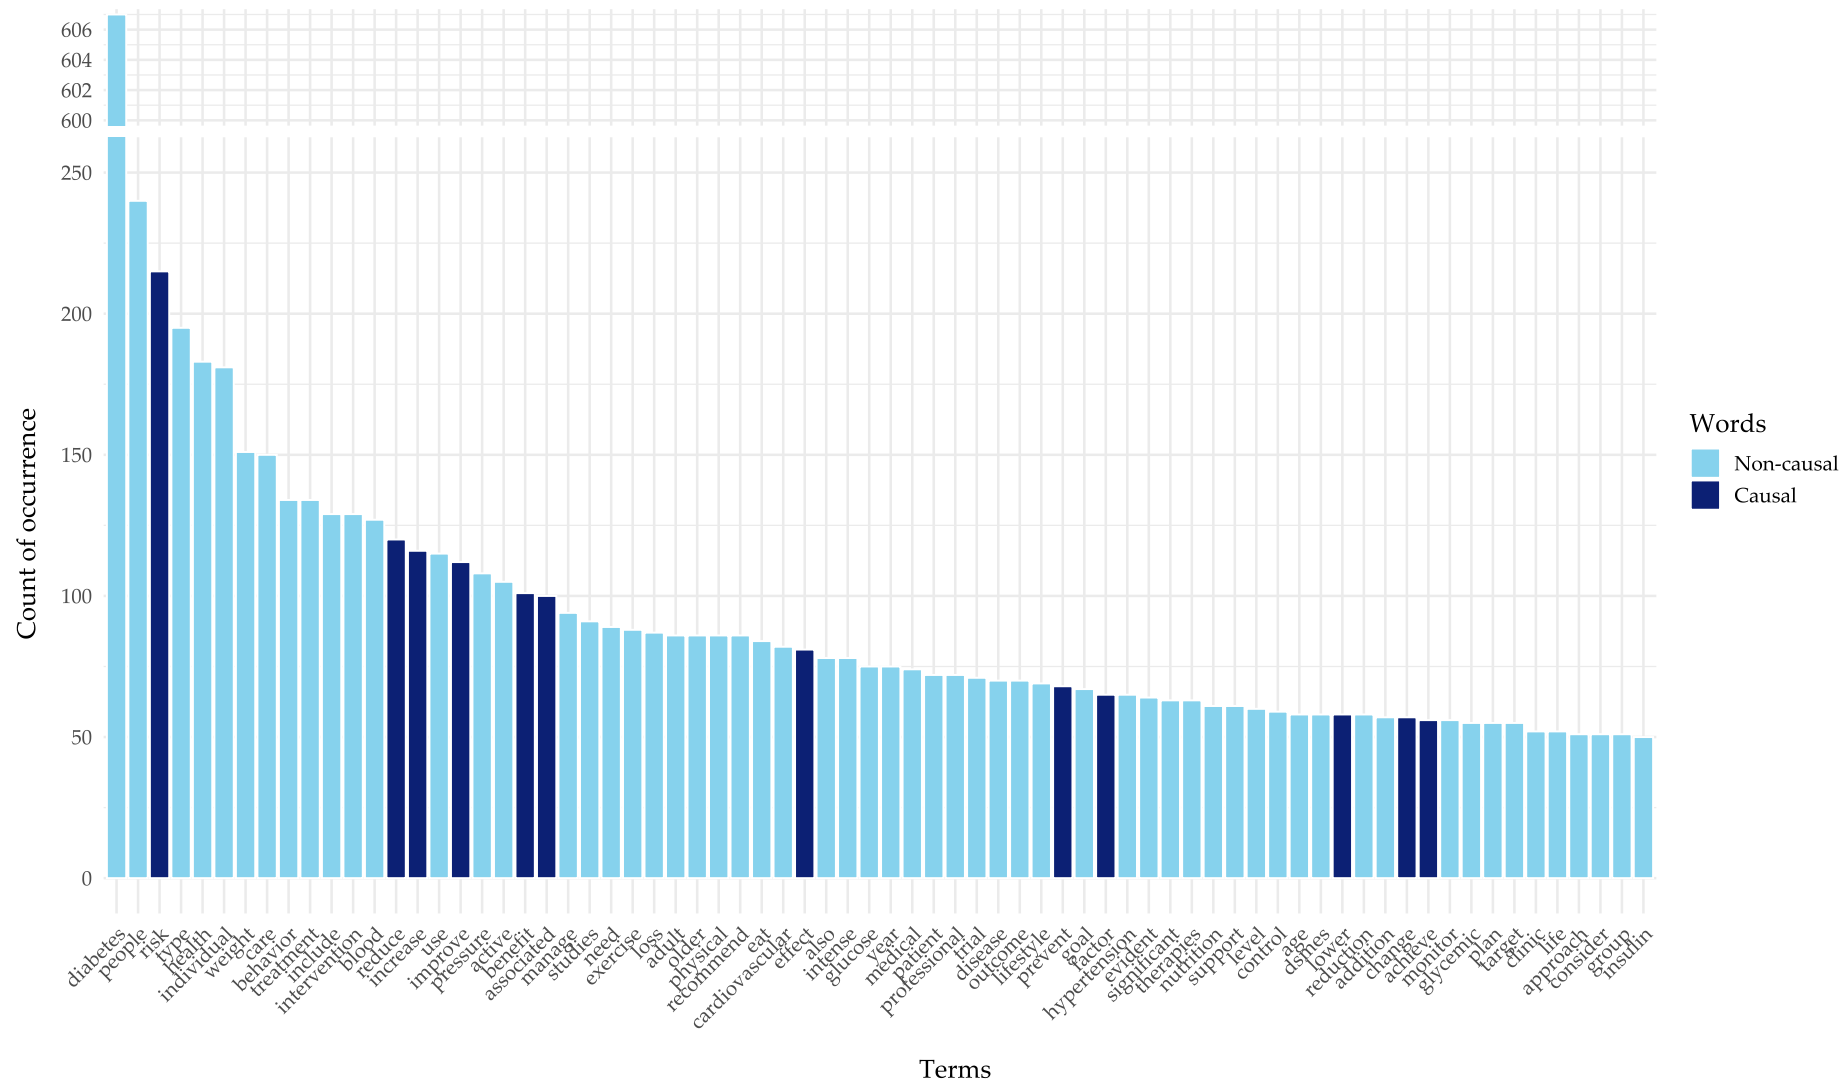

Figure S1.1: Count of occurrence of top-hit words in supporting statements. Only those appeared more than 50 times were included. Causal linking words were marked using the candidate list.

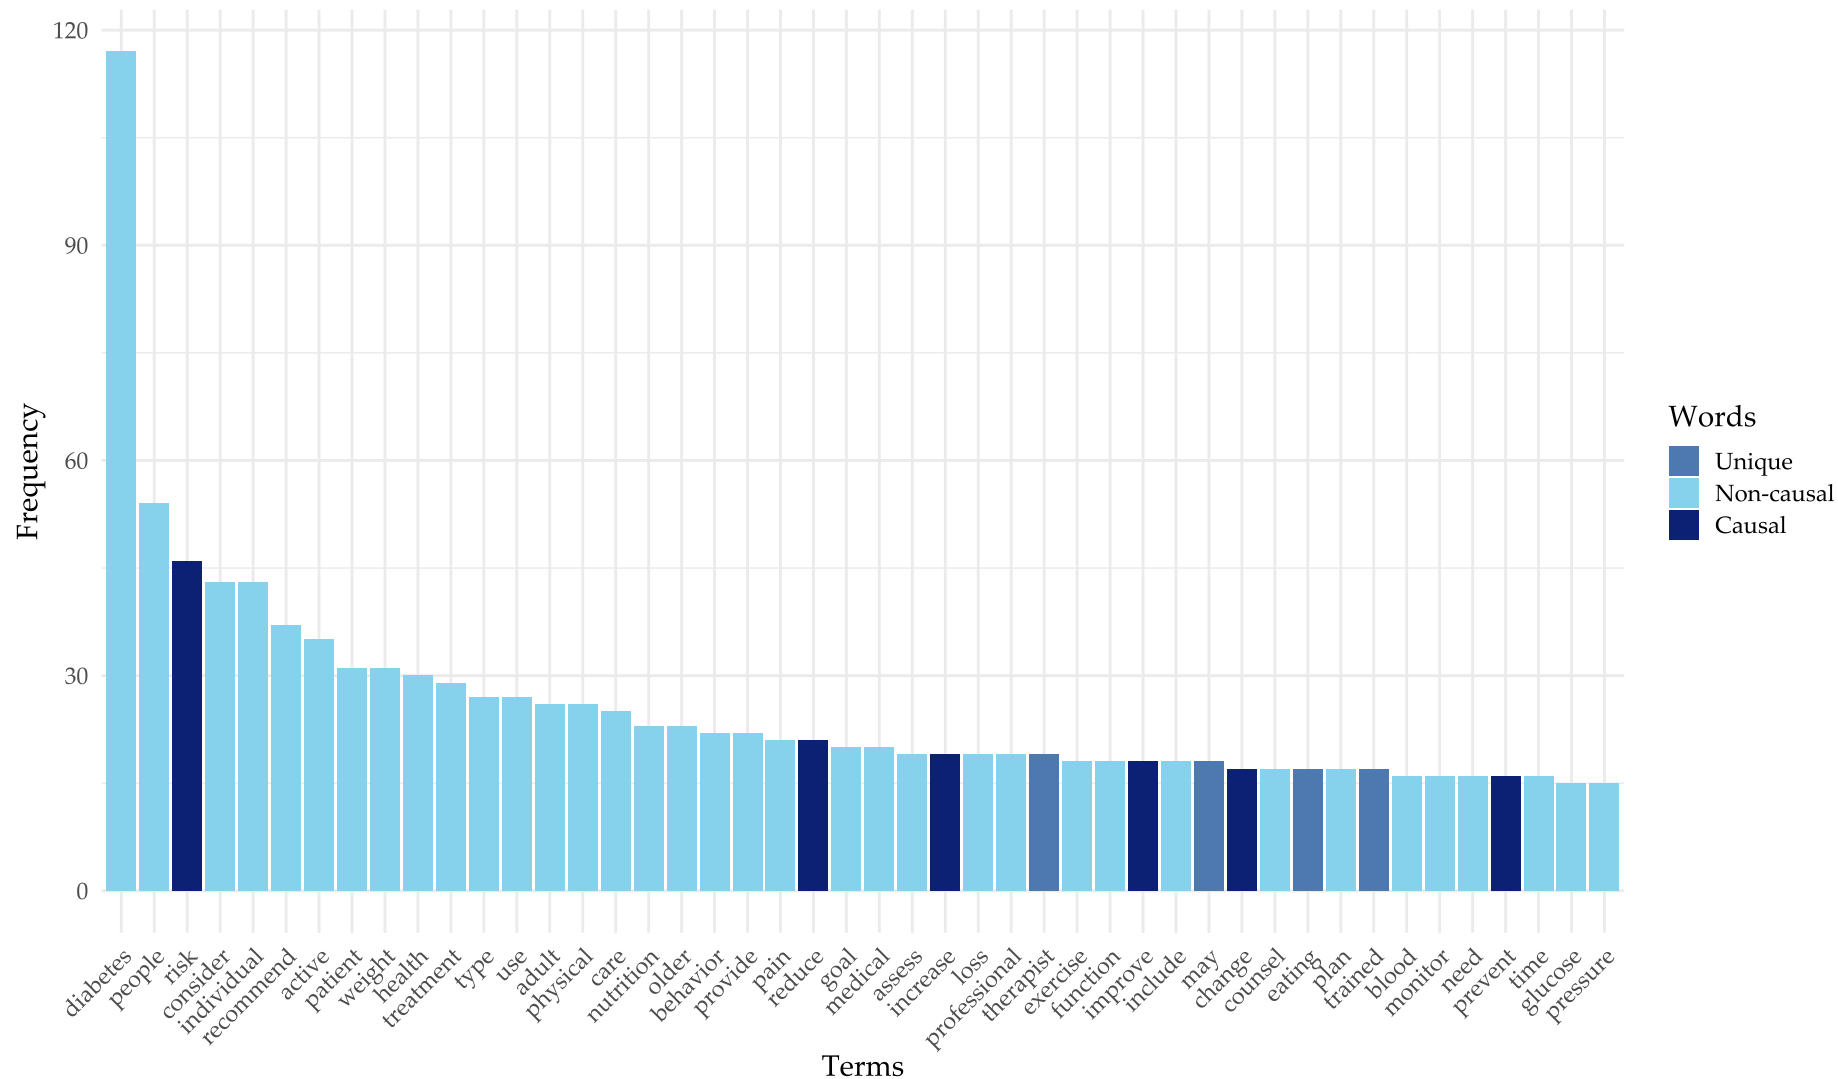

Figure S1.2: Count of occurrence of top-hit words in recommendation texts. Dark blue bars indicate candidate causal linking words; mid-blue bars for unique words in recommendation texts but not in supporting statements; and light-blue bar for other words.

# **File S2**

## **Details of scales used for rating**

This appendix contains details, rubrics and rater instructions for (1) *The Causal Implication Strength Rating Scale* and (2) the Target Trial Emulation (TTE) component reporting quality scale. This was used in the rating of guideline statements, original study sentences, and reporting quality.

### **S2.1 Scale for causation strength**

Table S2.1: The Causal Implication Strength Rating Scale for causation strength.

| Rating        | Description                                                                                                                                                                         | Linking word                                                                             | Modifier                                                                                                                                                                                                                  |
|---------------|-------------------------------------------------------------------------------------------------------------------------------------------------------------------------------------|------------------------------------------------------------------------------------------|---------------------------------------------------------------------------------------------------------------------------------------------------------------------------------------------------------------------------|
| 3<br>Strong   | The linking sentence clearly implies that causality had been identified.                                                                                                            | A linking word expressing strong explicit causation, <i>e.g.</i> “effect”, “beneficial”. | No weakening modifiers.                                                                                                                                                                                                   |
| 2<br>Moderate | The linking sentence mostly implies that a causal relationship was identified, but it is unclear or not possible to come to that conclusion in the absence of any causal inference. | A linking word expressing strong explicit causation, <i>e.g.</i> “effect”, “beneficial”. | One weakening modifier that weakens the tone or the expression of a sentence, <i>e.g.</i> “may”, “could”, “probably”                                                                                                      |
| 2<br>Moderate | Same as above                                                                                                                                                                       | A linking word expressing weak or implicit causation, <i>e.g.</i> “associated”, “risky”. | No weakening modifiers.                                                                                                                                                                                                   |
| 1<br>Weak     | The linking sentence might imply that a causal relationship was identified, but it is unclear or not possible to come to that conclusion in the absence of any causal inference.    | A linking word expressing strong explicit causation, <i>e.g.</i> “effect”, “beneficial”. | Several weakening modifiers that weaken the tone or the expression of a sentence, <i>e.g.</i> “may”, “could”, “probably”; Or the overall tone of the sentence expresses very weak confidence about the causation implied. |

Table S2.1 (Continued)

| Rating    | Description                                                                               | Linking word                                                                                           | Modifier                                                                                                                      |
|-----------|-------------------------------------------------------------------------------------------|--------------------------------------------------------------------------------------------------------|-------------------------------------------------------------------------------------------------------------------------------|
| 1<br>Weak | Same as above                                                                             | A linking word expressing weak or implicit causation, <i>e.g.</i> “associated”, “risky”.               | One or more weakening modifiers that weakens the tone or the expression of a sentence, <i>e.g.</i> “may”, “could”, “probably” |
| 0<br>None | The linking sentence does not imply in any way that a causal relationship was identified. | Note: The sentence still contains relationships between a set of variables or talks about correlation. | –                                                                                                                             |
| -1<br>N/A | –                                                                                         | Note: The sentence does not contain any variable relationships and is unrelated to correlation.        | –                                                                                                                             |

The description of this scale is modified from Haber et al. [7].

## S2.2 Scale for recommendation causation-dependence

Table S2.2: The Causal Implication Strength Rating Scale for causation-dependence of action recommendations

| Rating        | Description                                                                                                                                                                                                                | Explanation                                                                                                                           |
|---------------|----------------------------------------------------------------------------------------------------------------------------------------------------------------------------------------------------------------------------|---------------------------------------------------------------------------------------------------------------------------------------|
| 3<br>Strong   | The action recommendation could only be made appropriately had a causal relationship been identified.                                                                                                                      | We must make this recommendation based on new causal evidence; common knowledge sets are never sufficient to support it anymore.      |
| 2<br>Moderate | The action recommendation most likely could only be made appropriately had a causal relationship been identified, but it is unclear or not possible to come to that recommendation in the absence of any causal inference. | We need to make this recommendation based on new evidence, along with our common knowledge sets and subject-matter knowledge.         |
| 1<br>Weak     | The action recommendation may be made appropriately had a causal relationship been identified, but it is unclear or not possible to come to that recommendation in the absence of any causal inference.                    | We can make this recommendation with a little evidence and based on our common knowledge sets and subject-matter knowledge.           |
| 0<br>None     | The action recommendation would be made appropriately in the absence of any causal relationship.                                                                                                                           | We can make this recommendation in the absence of any evidence, only based on our common knowledge sets and subject-matter knowledge. |
| -1<br>N/A     | No action recommendation exists.                                                                                                                                                                                           | –                                                                                                                                     |

The description of this scale is modified from Haber et al. [7].

## S2.3 Scale for target trial emulation components

Table S2.3: The reporting quality scale for target trial emulation components

| TTE component        | Fully reported<br>(2/2)                                                                                                                                            | Partially reported<br>(1/2)                                                                                                                                                                        | Not reported<br>(0/2)                                                                                                                                                                                                                            |
|----------------------|--------------------------------------------------------------------------------------------------------------------------------------------------------------------|----------------------------------------------------------------------------------------------------------------------------------------------------------------------------------------------------|--------------------------------------------------------------------------------------------------------------------------------------------------------------------------------------------------------------------------------------------------|
| Eligibility criteria | Inclusion and exclusion criteria of participants are clearly given, or given in a protocol, prior to the description of the subsequent randomization and treatment | Inclusion and exclusion criteria are somewhat given, not clear enough, or given in brief. It requires additional judgements if one were to define the study population with the information given. | Only inclusion or exclusion criteria are given, and are in vast brief. Or that the eligibility criteria are reported along with participant selection or participant demographics/characteristics. It is very hard to define a study population. |
| Treatment strategies | [Interventional study]: treatment strategy is clearly given, with its time span, run-in or initiation, and procedures, which is replicable.                        | [Interventional study]: treatment strategy is given, but is not very detailed; time span, planned intervention sessions, monitoring, or some procedures could be not clear enough.                 | [Interventional study]: treatment strategy is very roughly described and cannot be replicated if asked to do so at all, or there is barrier from understanding how a treatment is carried out.                                                   |

Table S2.3 (Continued)

| TTE component         | Fully reported<br>(2/2)                                                                                                                                                                             | Partially reported<br>(1/2)                                                                                                                                               | Not reported<br>(0/2)                                                                                                                                                         |
|-----------------------|-----------------------------------------------------------------------------------------------------------------------------------------------------------------------------------------------------|---------------------------------------------------------------------------------------------------------------------------------------------------------------------------|-------------------------------------------------------------------------------------------------------------------------------------------------------------------------------|
|                       | [Observational study]: the definition of the exposure, as well as how and when it is measured, preferably also time span, is clearly given.                                                         | [Observational study]: at least one aspect mentioned in the left side is not clear enough or not reported.                                                                | [Observational study]: the definition of the exposure and how and when it is measured are unclear.                                                                            |
| Assignment procedures | [Randomized study]: The randomization procedure, including how block/stratum is constructed and with which method randomization is performed, needs to be described clearly.                        | [Randomized study]: The randomization is mentioned, but the specifications are not reported in detail.                                                                    | [Randomized study]: The study only claims that this is a randomized study, but any further information is not covered by the article text.                                    |
|                       | [Other study]: Covariate adjustment and between-group balance considerations before and after the [emulated] randomization time point should be discussed and appropriately conducted and reported. | Covariate adjustment and considerations about how to make groups comparable is mentioned but not in detail; rationale about the variables chosen is completely not given. | Covariate adjustment for group balance or the construction of a theoretical control for single-arm trials are not given or are given but are vast brief and very unjustified. |

Table S2.3 (Continued)

| TTE component       | Fully reported<br>(2/2)                                                                                                                                                                                                                          | Partially reported<br>(1/2)                                                                                                                                                                                                                                        | Not reported<br>(0/2)                                                                                                                                             |
|---------------------|--------------------------------------------------------------------------------------------------------------------------------------------------------------------------------------------------------------------------------------------------|--------------------------------------------------------------------------------------------------------------------------------------------------------------------------------------------------------------------------------------------------------------------|-------------------------------------------------------------------------------------------------------------------------------------------------------------------|
| Follow-up period    | The time zero, time span of follow-up, and the definition of the end of follow-up (if applicable) and the endpoint events that trigger ending follow-up, are clearly reported. Preferably, the time zero is explicitly stated in the study text. | The time span of follow-up is reported, but some information is missing, and it could be hard to replicate this study or reconstruct time at risks from raw data if one were to do so.                                                                             | The time span, risk period, or related considerations, are not reported. It is confused how the authors measured variables and/or decided to start/end follow-up. |
| Outcome of interest | The outcomes of interest are clearly defined. This includes the operationalized definition, how to measure it, and preferably the associated time span or a specific time point at which outcomes are measured.                                  | The outcomes of interest are partially reported; or only the primary outcome is given, while the information about the measurement of other outcomes is missing. It is hard to replicate this study's outcome measurement and calculation using information given. | The outcomes are very vaguely defined. It is nearly impossible to think about the procedure of outcome measurements and comparisons.                              |

Table S2.3 (Continued)

| TTE component   | Fully reported<br>(2/2)                                                                                                                                                                                                                                                                                                        | Partially reported<br>(1/2)                                                                                                                                                                           | Not reported<br>(0/2)                                                                                                                                                                 |
|-----------------|--------------------------------------------------------------------------------------------------------------------------------------------------------------------------------------------------------------------------------------------------------------------------------------------------------------------------------|-------------------------------------------------------------------------------------------------------------------------------------------------------------------------------------------------------|---------------------------------------------------------------------------------------------------------------------------------------------------------------------------------------|
| Causal contrast | The causal contrast, or the estimand, is clearly stated in the research question. This often appears at the very end of an introduction section of an article. The causal contrast includes: at least two treatment levels to be contrasted, an outcome that is clearly stated, time period, population, and other components. | The causal contrast or the estimand is somewhat expressed in the research question. There is not a clear sentence about the effect of interest, but traditional components – PICOS, are mostly given. | Although the study should be of a causal nature or of causal interests, the causal contrast, even the PICOS-components, are not clearly given or very badly expressed in the article. |

Table S2.3 (Continued)

| TTE component | Fully reported<br>(2/2)                                                                                                                                                                                                                                                                                                                                                                                  | Partially reported<br>(1/2)                                                                                                                                                                                      | Not reported<br>(0/2)                                                                                                                                                                                                                         |
|---------------|----------------------------------------------------------------------------------------------------------------------------------------------------------------------------------------------------------------------------------------------------------------------------------------------------------------------------------------------------------------------------------------------------------|------------------------------------------------------------------------------------------------------------------------------------------------------------------------------------------------------------------|-----------------------------------------------------------------------------------------------------------------------------------------------------------------------------------------------------------------------------------------------|
| Analysis plan | An analysis plan should be clearly presented, especially including 1 under which principle (ITT/PP/AT/CC) the analysis is carried out, and 2 how to deal with (emulated) post-randomization issues (loss to follow-up, nonadherence, contamination, etc.) For observational studies, adjustment for selection and losses to follow-up should be given, while ITT/PP principles need not to be mentioned. | An analysis plan is given, but at least one critical aspect is missing, such that it would be hard to replicate a complete data analysis procedure even with raw data, if only given the analysis plan reported. | The analysis plan is not given or very vague, and cannot provide any useful information that helps look into the implementation of actual data analysis. It is not possible to replicate a complete data analysis workflow as in the article. |

Abbreviations: PICOS, population, intervention, control, outcome, and study type; ITT, intention-to-treat; PP, per-protocol; AT, as-treated; CC, complete-case. The 3-item scale for reporting quality was derived from Smit et al. [8].

## S2.4 Examples for rating

In this section we give examples for each of the sentence ratings listed above and their rating considerations.

**Example 1: guideline statement causation rating** Disordered thinking and judgment can be expected to make it difficult to engage in behavior that reduces risk factors for type 2 diabetes, such as restrained eating for weight management.

- Causation rating: 1/3
- Considerations: (1) “make it difficult to engage” is a weak linking word that express some uncertainty; (2) “can be expected to” is a weakening modifier that make the sentence tone weaker with more uncertainty.

**Example 2: guideline statement causation rating** Potential adverse effects of antihypertensive therapy (e.g., hypotension, syncope, falls, AKI, and electrolyte abnormalities) should also be taken into account.

- Causation rating: 2/3
- Considerations: “adverse effects” is a strong causal linking word; however, “potential” is a modifier and adds to the uncertainty.

**Example 3: guideline statement causation rating** An RCT found that two meal-planning approaches (diabetes plate method and carbohydrate counting) were effective in helping achieve improved A1C.

- Causation rating: 3/3
- Considerations: “effective” is a strong causal linking word.

**Example 4: guideline recommendation causation-dependence** Monitor changes in body weight, glycemia, and lipids in adolescents and adults with diabetes who are prescribed second-generation antipsychotic medications; adjust the treatment plan accordingly, if needed.

- Causation-dependence rating: 0/3
- Considerations: This is more common sense and general practice; no novel evidence is necessary to support it.

**Example 5: guideline recommendation causation-dependence** Nutrition, physical activity, and behavioral therapy to achieve and maintain  $\geq 5\%$  weight loss are recommended for people with type 2 diabetes and overweight or obesity.

- Causation-dependence rating: 3/3

- Considerations: The goal of 5% weight loss is very specific and requires original studies that are dedicated to test for this percentage of weight loss to support, showing this is the optimal percentage.

**Example 6: content alignment between original studies and guideline statements** [Guideline] Therefore, other programs and modalities of behavioral counseling for diabetes prevention may also be appropriate and efficacious based on individual preferences and availability. [Original study] The percentage of participants retained through 18 weeks varied by age, race/ethnicity, mean weekly percentage of body weight lost, and mean weekly physical activity minutes but not by sex.

- Content alignment rating: 0/2
- Considerations: The guideline statement described the efficacy or “appropriateness”, while the original study conclusive sentence provided only information on attrition for one specific treatment.

**Example 7: content alignment between original studies and guideline statements** [Guideline] This benefit was greatest in people with diabetes. [Original study] In high-risk patients, there are additional benefits from more intensive blood pressure lowering.

- Content alignment rating: 1/2
- Considerations: (Combining with the context) the two sentences both talked about intensive blood pressure lowering strategies; however, the second one did not talk about whether this benefit was “greatest” in patients of higher risk of diabetes.



**File S3**

**Original study characteristics**

Table S3.1: Original study characteristics

| Title                                                                                                                                                                                   | Study type | First author            | Last author             | Year | Nationality | Journal                                    | Cited by | Cited by per year | Sampled |
|-----------------------------------------------------------------------------------------------------------------------------------------------------------------------------------------|------------|-------------------------|-------------------------|------|-------------|--------------------------------------------|----------|-------------------|---------|
| Diabetes and Hypertension: A Position Statement by the American Diabetes Association                                                                                                    | 7          | Ian H de Boer           | George Bakris           | 2017 | USA         | Diabetes Care                              | 852      | 106.5             | Yes     |
| Syncope, Hypotension, and Falls in the Treatment of Hypertension: Results from the Randomized Clinical Systolic Blood Pressure Intervention Trial                                       | 2          | Kaycee M. Sink          | Lawrence J. Fine        | 2018 | USA         | Journal of the American Geriatrics SOCIETY | 96       | 13.7              | Yes     |
| Blood Pressure Lowering in Type 2 Diabetes: A Systematic Review and Meta-analysis                                                                                                       | 5          | Connor A. Emdin         | Anushka Patel           | 2015 | GBR         | JAMA                                       | 1073     | 107.3             | Yes     |
| Trial of Intensive Blood-Pressure Control in Older Patients with Hypertension                                                                                                           | 1          | Weili Zhang             | Jun Cai                 | 2021 | CHN         | NEJM                                       | 462      | 115.5             | Yes     |
| Effects of Intensive Blood-Pressure Control in Type 2 Diabetes Mellitus                                                                                                                 | 1          | The AC-CORD Study Group | The AC-CORD Study Group | 2010 | USA         | NEJM                                       | 4340     | 289.3             | Yes     |
| Effects of intensive blood pressure lowering on cardiovascular and renal outcomes: updated systematic review and meta-analysis                                                          | 5          | Xinfang Xie             | Anthony Rodgers         | 2016 | CHN         | The Lancet                                 | 1192     | 132.4             | Yes     |
| Blood Pressure Targets in Subjects With Type 2 Diabetes Mellitus/Impaired Fasting Glucose: Observations From Traditional and Bayesian Random-Effects Meta-Analyses of Randomized Trials | 5          | Sripal Bangalore        | Franz H. Messerli       | 2011 | USA         | Circulation                                | 592      | 42.3              | Yes     |

Table S3.1 continued from previous page

| Title                                                                                                                                                                                                                                          | Study type | First author                  | Last author                   | Year | Nationality | Journal                               | Cited by | Cited by per year | Sampled |
|------------------------------------------------------------------------------------------------------------------------------------------------------------------------------------------------------------------------------------------------|------------|-------------------------------|-------------------------------|------|-------------|---------------------------------------|----------|-------------------|---------|
| Less-Tight versus Tight Control of Hypertension in Pregnancy                                                                                                                                                                                   | 1          | Laura Magee                   | A. Jean-Marie Moutquin        | 2015 | CAN         | NEJM                                  | 766      | 76.6              | Yes     |
| Effects on Blood Pressure of Reduced Dietary Sodium and the Dietary Approaches to Stop Hypertension (DASH) Diet                                                                                                                                | 1          | Frank Sacks                   | M. Jeffrey A. Cutler          | 2001 | USA         | NEJM                                  | 7179     | 299.1             | Yes     |
| 2014 Evidence-Based Guideline for the Management of High Blood Pressure in Adults: Report From the Panel Members Appointed to the Eighth Joint National Committee (JNC 8)                                                                      | 7          | Paul James                    | A. Eduardo Ortiz              | 2014 | USA         | JAMA                                  | 11691    | 1062.8            | Yes     |
| Effect of structured physical activity on prevention of major mobility disability in older adults: the LIFE study randomized clinical trial.                                                                                                   | 1          | Marco Pahor                   | Jeff D Williamson             | 2014 | USA         | JAMA                                  | 1560     | 141.8             | Yes     |
| Cardiovascular Effects of Intensive Lifestyle Intervention in Type 2 Diabetes                                                                                                                                                                  | 1          | The Look AHEAD Research Group | The Look AHEAD Research Group | 2013 | USA         | NEJM                                  | 3046     | 253.8             | Yes     |
| Association of the magnitude of weight loss and changes in physical fitness with long-term cardiovascular disease outcomes in overweight or obese people with type 2 diabetes: a post-hoc analysis of the Look AHEAD randomised clinical trial | 2          | The Look AHEAD Research Group | The Look AHEAD Research Group | 2016 | USA         | The Lancet Diabetes and Endocrinology | 11       | 1.2               | Yes     |

Table S3.1 continued from previous page

| Title                                                                                                                                                                                   | Study type | First author                               | Last author                                | Year | Nationality | Journal                               | Cited by | Cited by per year | Sampled |
|-----------------------------------------------------------------------------------------------------------------------------------------------------------------------------------------|------------|--------------------------------------------|--------------------------------------------|------|-------------|---------------------------------------|----------|-------------------|---------|
| Aging and physical function in type 2 diabetes: 8 years of an intensive lifestyle intervention                                                                                          | 2          | W. Jack Rejeski                            | Edward H. Ip                               | 2014 | USA         | The Journals of Gerontology Series A  | 63       | 5.7               | Yes     |
| Cognitive performance declines in older adults with type 1 diabetes: results from 32 years of follow-up in the DCCT and EDIC Study                                                      | 2          | Alan M Jacobson                            | John M Lachin                              | 2021 | USA         | The Lancet Diabetes and Endocrinology | 74       | 18.5              | Yes     |
| Long-term effects of lifestyle intervention or metformin on diabetes development and microvascular complications over 15-year follow-up: the Diabetes Prevention Program Outcomes Study | 2          | Diabetes Prevention Program Research Group | Diabetes Prevention Program Research Group | 2015 | USA         | The Lancet Diabetes and Endocrinology | 1021     | 102.1             | Yes     |
| Sustained reduction in the incidence of type 2 diabetes by lifestyle intervention: follow-up of the Finnish Diabetes Prevention Study                                                   | 2          | Jaana Lindström                            | Jaakko Tuomilehto                          | 2006 | FIN         | The Lancet                            | 2471     | 130.1             | Yes     |
| Clinical and Economic Impact of a Digital, Remotely-Delivered Intensive Behavioral Counseling Program on Medicare Beneficiaries at Risk for Diabetes and Cardiovascular Disease         | 3          | Fang Chen                                  | Timothy M. Dall                            | 2016 | USA         | PLoS One                              | 61       | 6.8               | Yes     |
| Retention Among Participants in the National Diabetes Prevention Program Lifestyle Change Program, 2012–2017                                                                            | 4          | Michael J. Cannon                          | Bryce D. Smith                             | 2020 | USA         | Diabetes Care                         | 111      | 22.2              | Yes     |

Table S3.1 continued from previous page

| Title                                                                                                                                                                                                | Study type | First author           | Last author        | Year | Nationality | Journal                                           | Cited by | Cited by per year | Sampled |
|------------------------------------------------------------------------------------------------------------------------------------------------------------------------------------------------------|------------|------------------------|--------------------|------|-------------|---------------------------------------------------|----------|-------------------|---------|
| Position of the Academy of Nutrition and Dietetics: the role of medical nutrition therapy and registered dietitian nutritionists in the prevention and treatment of prediabetes and type 2 diabetes. | 7          | Kathaleen Briggs Early | Kathleen Stanley   | 2018 | USA         | Journal of the Academy of Nutrition and Dietetics | 186      | 26.6              | Yes     |
| The Use of Language in Diabetes Care and Education                                                                                                                                                   | 7          | Jane K. Dickinson      | Martha M. Funnell  | 2017 | USA         | Diabetes Care                                     | 307      | 38.4              | Yes     |
| Self-management support in “real-world” settings: An empowerment-based intervention                                                                                                                  | 8          | Tricia S. Tang         | Jacob E. Kurlander | 2010 | USA         | Patient Education and Counseling                  | 294      | 19.6              | Yes     |
| Physical Activity of Moderate Intensity and Risk of Type 2 Diabetes: A systematic review                                                                                                             | 5          | Christie Y. Jeon       | Rob M. van Dam     | 2008 | USA         | Diabetes Care                                     | 1149     | 67.6              | Yes     |
| Weight-Loss Therapy in Type 2 Diabetes: Effects of Phentermine and Topiramate Extended Release                                                                                                       | 2          | W. Timothy Garvey      | Barbara Troupin    | 2014 | USA         | Diabetes Care                                     | 148      | 13.5              | Yes     |
| Development and validity of a 2-item screen to identify families at risk for food insecurity                                                                                                         | 4          | Erin R. Hager          | Deborah A. Frank   | 2010 | USA         | Pediatrics                                        | 1239     | 82.6              | Yes     |
| The diabetes nutrition education study randomized controlled trial: a comparative effectiveness study of approaches to nutrition in diabetes self-management education.                              | 1          | Michael E. Bowen       | Russell L. Rothman | 2016 | USA         | PATIENT EDUCATION AND COUNSELING                  | 136      | 15.1              | Yes     |

Table S3.1 continued from previous page

| Title                                                                                                                                                                                                                       | Study type | First author                          | Last author                           | Year | Nationality | Journal                                            | Cited by | Cited by per year | Sampled |
|-----------------------------------------------------------------------------------------------------------------------------------------------------------------------------------------------------------------------------|------------|---------------------------------------|---------------------------------------|------|-------------|----------------------------------------------------|----------|-------------------|---------|
| Behavioral approaches to nutrition and eating patterns for managing type 2 diabetes: A review                                                                                                                               | 7          | Meg Salvia                            | G. Paula A. Quatromoni                | 2023 | USA         | American Journal of Medicine Open                  | 14       | 7                 | Yes     |
| The Effect of Early Time-Restricted Eating vs Later Time-Restricted Eating on Weight Loss and Metabolic Health                                                                                                              | 5          | Juanhong Liu                          | Feng Liu                              | 2023 | CHN         | The Journal of Clinical Endocrinology & Metabolism | 28       | 14                | Yes     |
| Efficacy of low carbohydrate diet for type 2 diabetes mellitus management: A systematic review and meta-analysis of randomized controlled trials                                                                            | 5          | Yan Meng                              | Liyong Chen                           | 2017 | CHN         | Diabetes Research and Clinical Practice            | 284      | 35.5              | Yes     |
| Effects of Carbohydrate Counting on Glucose Control and Quality of Life Over 24 Weeks in Adult Patients With Type 1 Diabetes on Continuous Subcutaneous Insulin Infusion: A randomized, prospective clinical trial (GIOCAR) | 1          | Andrea Laurenzi                       | Marina Scavini                        | 2011 | ITA         | Diabetes Care                                      | 179      | 12.8              | Yes     |
| Nutrition Therapy for Adults With Diabetes or Prediabetes: A Consensus Report                                                                                                                                               | 6          | Alison B. Evert                       | William S. Yancy, Jr                  | 2019 | USA         | Diabetes Care                                      | 1290     | 215               | Yes     |
| Effects of n?3 Fatty Acid Supplements in Diabetes Mellitus                                                                                                                                                                  | 1          | The AS-CEND Study Collaborative Group | The AS-CEND Study Collaborative Group | 2018 | GBR         | NEJM                                               | 750      | 107.1             | Yes     |

Table S3.1 continued from previous page

| Title                                                                                                                                              | Study type | First author         | Last author            | Year | Nationality | Journal                                | Cited by | Cited by per year | Sampled |
|----------------------------------------------------------------------------------------------------------------------------------------------------|------------|----------------------|------------------------|------|-------------|----------------------------------------|----------|-------------------|---------|
| Cardiovascular Risk Reduction with Icosapent Ethyl for Hypertriglyceridemia                                                                        | 1          | Deepak L. Bhatt      | Christie M. Ballantyne | 2018 | USA         | NEJM                                   | 3015     | 430.7             | Yes     |
| A 12-week randomized clinical trial investigating the potential for sucralose to affect glucose homeostasis                                        | 1          | V. Lee Grotz         | J. Richard Trout       | 2017 | USA         | Regulatory Toxicology and Pharmacology | 95       | 11.9              | Yes     |
| 2018 Physical Activity Guidelines Advisory Committee Scientific Report                                                                             | 7          | Abby C. King         | Abby C. King           | 2018 | USA         | .                                      | .        | .                 | Yes     |
| The Effects of Text Messages for Promoting Physical Activities in Prediabetes: A Randomized Controlled Trial                                       | 1          | Prawit Bootwong      | Nirun Intarut          | 2022 | THA         | Telemedicine and e-Health              | 9        | 3                 | Yes     |
| Physical Activity and Mortality in Individuals With Diabetes Mellitus: A Prospective Study and Meta-analysis                                       | 5          | Diewertje Sluik      | Ute Nöthlings          | 2012 | DEU         | JAMA Internal Medicine                 | 427      | 32.8              | Yes     |
| Physical fitness and activity changes after a 24-week soccer-based adaptation of the U.S diabetes prevention program intervention in Hispanic men  | 8          | Jennifer K. Frediani | Felipe Lobelo          | 2020 | USA         | Progress in Cardiovascular Diseases    | 21       | 4.2               | Yes     |
| Physical Activity/Exercise and Diabetes: A Position Statement of the American Diabetes Association                                                 | 7          | Sheri R. Colberg     | Deborah F. Tate        | 2016 | USA         | Diabetes Care                          | 3106     | 345.1             | Yes     |
| Acute high-intensity interval exercise reduces the postprandial glucose response and prevalence of hyperglycaemia in patients with type 2 diabetes | 8          | J. B. Gillen         | M. J. Gibala           | 2012 | CAN         | Diabetes, Obesity and Metabolism       | 398      | 30.6              | Yes     |

Table S3.1 continued from previous page

| Title                                                                                                                                                                      | Study type | First author                                                                                          | Last author                                                                                           | Year    | Nationality | Journal                               | Cited by | Cited by per year | Sampled |
|----------------------------------------------------------------------------------------------------------------------------------------------------------------------------|------------|-------------------------------------------------------------------------------------------------------|-------------------------------------------------------------------------------------------------------|---------|-------------|---------------------------------------|----------|-------------------|---------|
| Clinical outcomes and glycaemic responses to different aerobic exercise training intensities in type II diabetes: a systematic review and meta-analysis                    | 5          | Aimee Grace                                                                                           | Neil Smart                                                                                            | A. 2017 | AUS         | Cardiovascular Diabetology            | 195      | 24.4              | Yes     |
| Leisure-Time Running Reduces the Risk of Incident Type 2 Diabetes                                                                                                          | 3          | Yuehan Wang                                                                                           | Steven Blair                                                                                          | N 2019  | NLD         | The American Journal of Medicine      | 42       | 7                 | Yes     |
| The health consequences of smoking—50 years of progress: a report of the Surgeon General                                                                                   | 7          | National Center for Chronic Disease Prevention and Health Promotion (US) Office on Smoking and Health | National Center for Chronic Disease Prevention and Health Promotion (US) Office on Smoking and Health | 2014    | USA         | .                                     | .        | .                 | Yes     |
| Relation of active, passive, and quitting smoking with incident type 2 diabetes: a systematic review and meta-analysis                                                     | 5          | An Pan                                                                                                | Tangchun Wu                                                                                           | 2015    | CHN         | The Lancet Diabetes and Endocrinology | 596      | 59.6              | Yes     |
| Impact of Smokeless Tobacco Products on Cardiovascular Disease: Implications for Policy, Prevention, and Treatment: A Policy Statement From the American Heart Association | 6          | Mariann R. Piano                                                                                      | George Howard                                                                                         | 2010    | USA         | Circulation                           | 290      | 19.3              | Yes     |

Table S3.1 continued from previous page

| Title                                                                                                                                                         | Study type | First author        | Last author              | Year | Nationality | Journal                                                     | Cited by | Cited by per year | Sampled |
|---------------------------------------------------------------------------------------------------------------------------------------------------------------|------------|---------------------|--------------------------|------|-------------|-------------------------------------------------------------|----------|-------------------|---------|
| Prospective, Cluster-Randomized Trial to Implement the Ottawa Model for Smoking Cessation in Diabetes Education Programs in Ontario, Canada                   | 1          | Robert Reid         | D. Andrew L. Pipe        | 2018 | CAN         | Diabetes Care                                               | 26       | 3.7               | Yes     |
| Interventions With Adherence-Promoting Components in Pediatric Type 1 Diabetes: Meta-analysis of their impact on glycemic control                             | 5          | Korey Hood          | K. Dennis Dro-<br>tar    | 2010 | USA         | Diabetes Care                                               | 224      | 14.9              | Yes     |
| Applying Behavioral Economics Theories to Interventions for Persons with Diabetes                                                                             | 7          | Susana Patton       | R. Amy Hughes<br>Lansing | 2022 | USA         | Current Dia-<br>betes Reports                               | 8        | 2.7               | Yes     |
| Cost-effectiveness of three doses of a behavioral intervention to prevent or delay type 2 diabetes in rural areas                                             | 2          | Tiffany Radcliff    | A. Michael G. Perri      | 2020 | USA         | Journal of the Academy of Nu-<br>trition and Di-<br>etetics | 15       | 3                 | Yes     |
| Evaluation of the Effects of 12 Weeks Mindfulness-Based Stress Reduction on Glycemic Control and Mental Health Indices in Women with Diabetes Mellitus Type 2 | 1          | Omid Nikkhah Ravari | Anahita Babak            | 2020 | IRA         | Advanced Biomedical Research                                | 18       | 3.6               | Yes     |
| Psychosocial outcomes in young adolescents with type 1 diabetes participating in shared medical appointments                                                  | 1          | Shideh Majidi       | Jennifer K. Raymond      | 2021 | USA         | Pediatric Dia-<br>betes                                     | 14       | 3.5               | Yes     |

Table S3.1 continued from previous page

| Title                                                                                                                                                                                           | Study type | First author        | Last author            | Year | Nationality | Journal                      | Cited by | Cited by per year | Sampled |
|-------------------------------------------------------------------------------------------------------------------------------------------------------------------------------------------------|------------|---------------------|------------------------|------|-------------|------------------------------|----------|-------------------|---------|
| Effects of mindfulness- and acceptance-based interventions on diabetes distress and glycaemic level in people with type 2 diabetes: systematic review and meta-analysis.                        | 5          | Hau Ngan            | Yi Wai Tong Chien      | 2021 | HKG         | DIABETIC MEDICINE            | 62       | 15.5              | Yes     |
| Kindness Matters: A Randomized Controlled Trial of a Mindful Self-Compassion Intervention Improves Depression, Distress, and HbA1c Among Patients With Diabetes                                 | 1          | Anna Friis          | M. Nathan S. Consedine | 2016 | NZL         | Diabetes Care                | 301      | 33.4              | Yes     |
| Improving Quality Outcomes: The Value of Diabetes Care and Education Specialists                                                                                                                | 7          | Kellie Rodriguez    | Victor Phan            | 2022 | USA         | Clinical Diabetes            | 26       | 8.7               | Yes     |
| Related factors associated with fear of hypoglycemia in parents of children and adolescents with type 1 diabetes - A systematic review                                                          | 6          | Lu Zhang            | Yu Zhang               | 2022 | CHN         | Journal of Pediatric Nursing | 23       | 7.7               | Yes     |
| Effect of a collaborative care model on anxiety symptoms among patients with depression and diabetes in India: The INDEPENDENT randomized clinical trial                                        | 2          | Christopher G. Kemp | Lydia A. Chwastiak     | 2022 | IND         | General Hospital Psychiatry  | 21       | 7                 | Yes     |
| Cognitive behavior therapy for diabetes distress, depression, health anxiety, quality of life and treatment adherence among patients with type-II diabetes mellitus: a randomized control trial | 1          | Qasir Abbas         | Washdev Washdev        | 2023 | PAK         | BMC Psychiatry               | 30       | 15                | Yes     |

Table S3.1 continued from previous page

| Title                                                                                                                                                                                        | Study type | First author                  | Last author        | Year | Nationality | Journal                                            | Cited by | Cited by per year | Sampled |
|----------------------------------------------------------------------------------------------------------------------------------------------------------------------------------------------|------------|-------------------------------|--------------------|------|-------------|----------------------------------------------------|----------|-------------------|---------|
| Lifetime Duration of Depressive Disorders in Patients With Type 2 Diabetes                                                                                                                   | 8          | Mary de Groot                 | Jay H. Shubrook    | 2016 | USA         | Diabetes Care                                      | 68       | 7.6               | Yes     |
| The Pathways Study: A Randomized Trial of Collaborative Care in Patients With Diabetes and Depression                                                                                        | 1          | Wayne J. Katon                | Terry Bush         | 2004 | USA         | JAMA Psychiatry                                    | 928      | 44.2              | Yes     |
| The Effect of Exercise Interventions to Improve Psychosocial Aspects and Glycemic Control in Type 2 Diabetic Patients: A Systematic Review and Meta-Analysis of Randomized Controlled Trials | 5          | Gholam Rasul Moham-mad Rahimi | Vahid Saatchian    | 2021 | IRA         | Biological Research For Nursing                    | 7        | 1.8               | Yes     |
| The association between type 2 diabetes and attention- deficit/hyperactivity disorder: A systematic review, meta-analysis, and population-based sibling study                                | 5          | Miguel Garcia-Argibay         | Henrik Larsson     | 2023 | SWE         | Neuroscience and Biobehavioral Reviews             | 20       | 10                | Yes     |
| Severe Hypoglycemia and Cognitive Decline in Older People With Type 2 Diabetes: The Edinburgh Type 2 Diabetes Study                                                                          | 3          | Insa Feinkohl                 | Jackie F. Price    | 2014 | GBR         | Diabetes Care                                      | 318      | 28.9              | Yes     |
| A Diabetes Mobile App With In-App Coaching From a Certified Diabetes Educator Reduces A1C for Individuals With Type 2 Diabetes                                                               | 8          | Shefali Kumar                 | Jessie L. Ju-usola | 2018 | USA         | The Science of Diabetes Self-Management and Care   | 82       | 11.7              | Yes     |
| Digital Coaching Strategies to Facilitate Behavioral Change in Type 2 Diabetes: A Systematic Review                                                                                          | 6          | Bradley D Ger-shkowitz        | Bradley H Crotty   | 2021 | USA         | The Journal of Clinical Endocrinology & Metabolism | 32       | 8                 | Yes     |

Table S3.1 continued from previous page

| Title                                                                                                                                                                            | Study type | First author                      | Last author           | Year | Nationality | Journal                                    | Cited by | Cited by per year | Sampled |
|----------------------------------------------------------------------------------------------------------------------------------------------------------------------------------|------------|-----------------------------------|-----------------------|------|-------------|--------------------------------------------|----------|-------------------|---------|
| Impact of flash glucose Monitoring in people with type 2 Diabetes Inadequately controlled with non-insulin Antihyperglycaemic Therapy (IMMEDIATE): A randomized controlled trial | 1          | Ronnie Aronson                    | Ronald Goldenberg     | 2022 | CAN         | Diabetes, Obesity and Metabolism           | 48       | 16                | Yes     |
| Impact of Shift Work on Glycemic Control in Insulin Treated Diabetics Dar El Chefa Hospital                                                                                      | 4          | Ihab Mohammadi El Tayeb           | Basma Kamal Ramadan   | 2014 | EGY         | International Journal of Diabetes Research | 10       | 0.9               | Yes     |
| Sleep interventions and glucose metabolism: systematic review and meta-analysis                                                                                                  | 5          | Vallari Kothari                   | Sirimon Reutrakul     | 2021 | USA         | Sleep Medicine                             | 49       | 12.3              | Yes     |
| Learning in a Virtual Environment to Improve Type 2 Diabetes Outcomes: Randomized Controlled Trial                                                                               | 1          | Constance M Johnson               | Allison Vorderstrasse | 2022 | USA         | JMIR Formative Research                    | 8        | 2.7               | Yes     |
| The management of very low-calorie ketogenic diet in obesity outpatient clinic: a practical guide                                                                                | 7          | Giovanna Muscogiuri, Luigi Barrea | Annamaria Colao       | 2019 | ITA         | Journal of Translational Medicine          | 163      | 27.2              | Yes     |
| The Evolution of Very-Low-Calorie Diets: An Update and Meta-analysis                                                                                                             | 5          | Adam Gilden Tsai                  | Thomas A. Wadden      | 2012 | USA         | Obesity                                    | 538      | 41.4              | Yes     |
| Efficacy of dietary supplements containing isolated organic compounds for weight loss: a systematic review and meta-analysis of randomised placebo-controlled trials             | 5          | Erica Bessell                     | Nicholas R. Fuller    | 2021 | AUS         | International Journal of Obesity           | 16       | 4                 | Yes     |

| Table S3.1 continued from previous page                                                                                                                                                                                                                            |            |                                            |    |                                            |   |      |             |                                                    |          |                   |         |  |
|--------------------------------------------------------------------------------------------------------------------------------------------------------------------------------------------------------------------------------------------------------------------|------------|--------------------------------------------|----|--------------------------------------------|---|------|-------------|----------------------------------------------------|----------|-------------------|---------|--|
| Title                                                                                                                                                                                                                                                              | Study type | First author                               |    | Last author                                |   | Year | Nationality | Journal                                            | Cited by | Cited by per year | Sampled |  |
| Impact of weight loss on waist circumference and the components of the metabolic syndrome                                                                                                                                                                          | 8          | Amy                                        | E  | William                                    | H | 2017 | USA         | BMJ Open Diabetes Research and Care                | 107      | 13.4              | Yes     |  |
| Reduction in the Incidence of Type 2 Diabetes with Lifestyle Intervention or Metformin                                                                                                                                                                             | 1          | Diabetes Prevention Program Research Group |    | Diabetes Prevention Program Research Group |   | 2002 | USA         | NEJM                                               | 25615    | 1113.7            | Yes     |  |
| 2017 ACC/AHA/HFSA Focused Update of the 2013 ACCF/AHA Guideline for the Management of Heart Failure: A Report of the American College of Cardiology/American Heart Association Task Force on Clinical Practice Guidelines and the Heart Failure Society of America | 6          | Clyde                                      | W. | Cheryl                                     |   | 2017 | USA         | Circulation                                        | 5841     | 730.1             | Yes     |  |
| Cardiovascular Effects of Intensive Lifestyle Intervention in Type 2 Diabetes                                                                                                                                                                                      | 1          | The Look AHEAD Research Group              |    |                                            |   | 2013 | USA         | NEJM                                               | 3046     | 253.8             | Yes     |  |
| The efficacy and safety of meal replacement in patients with type 2 diabetes.                                                                                                                                                                                      | 5          | Wenjing Ye                                 |    | Liehua Liu                                 |   | 2023 | CHN         | The Journal of Clinical Endocrinology & Metabolism | 8        | 4                 | Yes     |  |
| 10-Year Follow-up of Intensive Glucose Control in Type 2 Diabetes                                                                                                                                                                                                  | 2          | Rury                                       | R. | H. Andrew                                  |   | 2008 | GBR         | NEJM                                               | 10257    | 603.4             | Yes     |  |

Table S3.1 continued from previous page

| Title                                                                                                                                                                                      | Study type | First author          | Last author               | Year | Nationality | Journal                                                                             | Cited by | Cited by per year | Sampled |
|--------------------------------------------------------------------------------------------------------------------------------------------------------------------------------------------|------------|-----------------------|---------------------------|------|-------------|-------------------------------------------------------------------------------------|----------|-------------------|---------|
| Years of life gained by multifactorial intervention in patients with type 2 diabetes mellitus and microalbuminuria: 21 years follow-up on the Steno-2 randomised trial                     | 2          | Peter Gæde            | Oluf Peder-<br>sen        | 2016 | DNK         | DIABETOLOGIA                                                                        | 1        | 0.1               | Yes     |
| Effect of early intensive multifactorial therapy on 5-year cardiovascular outcomes in individuals with type 2 diabetes detected by screening (ADDITION-Europe): a cluster-randomised trial | 1          | Simon Griffin         | J Torsten<br>Lauritzen    | 2011 | GBR         | The Lancet                                                                          | 569      | 40.6              | Yes     |
| Treatment intensification with stepwise addition of prandial insulin aspart boluses compared with full basal-bolus therapy (FullSTEP Study): a randomised, treat-to-target clinical trial  | 1          | Helena Rodbard        | W David<br>HW Shu         | 2014 | USA         | The Lancet Di-<br>abetes and En-<br>docrinology                                     | 118      | 10.7              | Yes     |
| The Effects of Dietary Education Interventions on Individuals with Type 2 Diabetes: A Systematic Review and Meta-Analysis                                                                  | 5          | Juri Kim              | Myung-<br>Haeng<br>Hur    | 2021 | KOR         | International<br>Journal of En-<br>vironmental<br>Research and<br>Public Health ... | 24       | 6                 | Yes     |
| Cardiorespiratory Fitness, BMI, Mortality, and Cardiovascular Disease in Adults with Overweight/Obesity and Type 2 Diabetes                                                                | 2          | WILLS,<br>ANDREW<br>C | KNOWLER,<br>WILLIAM<br>C. | 2021 | USA         | Medicine & Sci-<br>ence in Sports &<br>Exercise                                     | 7        | 1.8               | Yes     |

Table S3.1 continued from previous page

| Title                                                                                                                                                                                                             | Study type | First author         | Last author           | Year | Nationality | Journal                                       | Cited by | Cited by per year | Sampled |
|-------------------------------------------------------------------------------------------------------------------------------------------------------------------------------------------------------------------|------------|----------------------|-----------------------|------|-------------|-----------------------------------------------|----------|-------------------|---------|
| Lifestyle Intervention and Medical Management With vs Without Roux-en-Y Gastric Bypass and Control of Hemoglobin A1c, LDL Cholesterol, and Systolic Blood Pressure at 5 Years in the Diabetes Surgery Study       | 2          | Sayeed Ikramuddin    | Charles J. Billington | 2018 | USA         | JAMA                                          | 307      | 43.9              | Yes     |
| Long-term secondary prevention of cardiovascular disease with a Mediterranean diet and a low-fat diet (CORDIOPREV): a randomised controlled trial                                                                 | 1          | Javier Delgado-Lista | Jose Lopez-Miranda    | 2022 | ESP         | The Lancet                                    | 316      | 105.3             | Yes     |
| Nutrition Therapy Recommendations for the Management of Adults With Diabetes                                                                                                                                      | 7          | Alison B. Evert      | William S. Yancy      | 2013 | USA         | Diabetes Care                                 | 2135     | 177.9             | Yes     |
| Salt Reduction to Prevent Hypertension and Cardiovascular Disease: JACC State-of-the-Art Review                                                                                                                   | 5          | Feng J. He           | Graham A. MacGregor   | 2020 | GBR         | Journal of the American College of Cardiology | 472      | 94.4              | Yes     |
| Association between Bout Duration of Physical Activity and Health: Systematic Review                                                                                                                              | 6          | John M Jakicic       | Katrina L Piercy      | 2018 | USA         | Medicine & Science in Sports & Exercise       | 281      | 40.1              | Yes     |
| Are physical activity interventions for healthy inactive adults effective in promoting behavior change and maintenance, and which behavior change techniques are effective? A systematic review and meta-analysis | 5          | Neil Howlett         | Angel Marie Chater    | 2018 | GBR         | Translational Behavioral Medicine             | 378      | 54                | Yes     |

Table S3.1 continued from previous page

| Title                                                                                                                             | Study type | First author                   | Last author        | Year | Nationality | Journal                                    | Cited by | Cited by per year | Sampled |
|-----------------------------------------------------------------------------------------------------------------------------------|------------|--------------------------------|--------------------|------|-------------|--------------------------------------------|----------|-------------------|---------|
| Effectiveness of medical nutrition therapy in diabetes.                                                                           | 6          | Pastors JG                     | Franz MJ           | 2012 | USA         | .                                          | 24       | 1.8               | Yes     |
| Effects of exercise on glycemic control and body mass in type 2 diabetes mellitus. A meta-analysis of controlled clinical trials. | 5          | Normand G. Boulé               | Ronald J. Sigal    | 2001 | CAN         | JAMA                                       | 2984     | 124.3             | Yes     |
| Bariatric surgery: an IDF statement for obese Type 2 diabetes                                                                     | 7          | J. B. Dixon                    | F. Rubino          | 2011 | AUS         | DIABETIC MEDICINE                          | 953      | 68.1              | Yes     |
| Association between body mass index and mortality in an 80-year-old population                                                    | 3          | Yutaka Takata                  | Tadamichi Takehara | 2007 | JPN         | JOURNAL OF THE AMERICAN GERIATRICS SOCIETY | 92       | 5.1               | Yes     |
| Effect of Weight Loss and Exercise on Frailty in Obese Older Adults                                                               | 1          | Dennis T. Villareal            | David R. Sinacore  | 2006 | USA         | JAMA Internal Medicine                     | 389      | 20.5              | Yes     |
| Clinical Effectiveness of First and Repeat Influenza Vaccination in Adult and Elderly Diabetic Patients                           | 4          | Ingrid Looijmans-Van den Akker | Eelko Hak          | 2006 | NLD         | Diabetes Care                              | 167      | 8.8               | Yes     |
| Brain Morphological Signatures for Chronic Pain                                                                                   | 4          | Marwan N. Baliki               | A. Vania Apkarian  | 2011 | USA         | PLoS One                                   | 441      | 31.5              | Yes     |
| Pain Assessment and Management in Aging                                                                                           | 7          | Mimi Hanks-Bell                | Judith A. Paice    | 2004 | USA         | Online Journal of Issues in Nursing        | 61       | 2.9               | Yes     |

Table S3.1 continued from previous page

| Title                                                                                                                                                                              | Study type | First author              | Last author               | Year | Nationality | Journal                                 | Cited by | Cited by per year | Sampled |
|------------------------------------------------------------------------------------------------------------------------------------------------------------------------------------|------------|---------------------------|---------------------------|------|-------------|-----------------------------------------|----------|-------------------|---------|
| Efficacy of treating pain to reduce behavioural disturbances in residents of nursing homes with dementia: cluster randomised clinical trial                                        | 1          | Bettina Husebo            | S Dag Aarsland            | 2011 | NOR         | BMJ                                     | 671      | 47.9              | Yes     |
| A randomized trial of intensive versus standard blood-pressure control                                                                                                             | 1          | The SPRINT Research Group | The SPRINT Research Group | 2015 | USA         | NEJM                                    | 6553     | 655.3             | No      |
| Effects of intensive blood-pressure control in type 2 diabetes mellitus                                                                                                            | 1          | ACCORD Study Group        | ACCORD Study Group        | 2010 | USA         | NEJM                                    | 4410     | 294               | No      |
| Intensive systolic blood pressure control and incident chronic kidney disease in people with and without diabetes mellitus: secondary analyses of two randomised controlled trials | 2          | Srinivasan Beddhu         | Glenn M Chertow           | 2018 | USA         | The Lancet Diabetes and Endocrinology   | 110      | 15.71             | No      |
| Blood pressure targets for hypertension in people with diabetes mellitus                                                                                                           | 5          | Jose Agustin Arguedas     | James M Wright            | 2013 | CRI         | Cochrane Database of Systematic reviews | 240      | 20                | No      |
| Blood pressure lowering for prevention of cardiovascular disease and death: a systematic review and meta-analysis                                                                  | 5          | Dena Ettehad              | Kazem Rahimi              | 2016 | GBR         | The Lancet                              | 4200     | 466.67            | No      |

Table S3.1 continued from previous page

| Title                                                                                                                                                                                                                                       | Study type | First author        | Last author        | Year | Nationality | Journal                                    | Cited by | Cited by per year | Sampled |
|---------------------------------------------------------------------------------------------------------------------------------------------------------------------------------------------------------------------------------------------|------------|---------------------|--------------------|------|-------------|--------------------------------------------|----------|-------------------|---------|
| Effect of antihypertensive treatment at different blood pressure levels in patients with diabetes mellitus: systematic review and meta-analyses                                                                                             | 5          | Mattias Brunström   | Bo Carlberg        | 2016 | SWE         | BMJ                                        | 509      | 56.56             | No      |
| Blood Pressure Targets in Subjects With Type 2 Diabetes Mellitus/Impaired Fasting Glucose: Observations From Traditional and Bayesian Random-Effects Meta-Analyses of Randomized Trials                                                     | 5          | Sripal Bangalore    | Franz H. Messerli  | 2011 | USA         | Circulation                                | 598      | 42.71             | No      |
| Effects of blood-pressure-lowering treatment on outcome incidence in hypertension 10 – Should blood pressure management differ in hypertensive patients with and without diabetes mellitus? Overview and meta-analyses of randomized trials | 5          | Thomopoulos, Costas | Zanchetti, Alberto | 2017 | GRC         | Journal of Hypertension                    | 304      | 38                | No      |
| Effects of intensive blood pressure lowering on cardiovascular and renal outcomes: updated systematic review and meta-analysis                                                                                                              | 5          | Xinfang Xie         | Anthony Rodgers    | 2016 | CHN         | The Lancet                                 | 1232     | 136.89            | No      |
| A Program to Prevent Functional Decline in Physically Frail, Elderly Persons Who Live at Home                                                                                                                                               | 1          | Thomas M. Gill      | Amy Byers          | 2002 | USA         | NEJM                                       | 1160     | 50.43             | No      |
| Intensive Weight Loss Intervention in Older Individuals: Results from the Action for Health in Diabetes Type 2 Diabetes Mellitus Trial                                                                                                      | 1          | Mark A. Espeland    | Helen P. Hazuda    | 2013 | USA         | Journal of the American Geriatrics Society | 79       | 6.58              | No      |

Table S3.1 continued from previous page

| Title                                                                                                                                                                                                             | Study type | First author      | Last author      | Year    | Nationality | Journal                               | Cited by | Cited by per year | Sampled |
|-------------------------------------------------------------------------------------------------------------------------------------------------------------------------------------------------------------------|------------|-------------------|------------------|---------|-------------|---------------------------------------|----------|-------------------|---------|
| Severe hypoglycemia and cognitive decline in older people with type 2 diabetes: the Edinburgh type 2 diabetes study                                                                                               | 3          | Insa Feinkohl     | Jackie Price     | F. 2014 | GBR         | Diabetes Care                         | 327      | 29.73             | No      |
| Severe hypoglycaemia, mild cognitive impairment, dementia and brain volumes in older adults with type 2 diabetes: the Atherosclerosis Risk in Communities (ARIC) cohort study                                     | 3          | Alexandra K. Lee  | Elizabeth Selvin | 2018    | USA         | Diabetologia                          | 103      | 14.71             | No      |
| Reduction in the incidence of type 2 diabetes with lifestyle intervention or metformin                                                                                                                            | 1          | William C Knowler | David M Nathan   | 2002    | USA         | NEJM                                  | 25978    | 1129.48           | No      |
| Cardiovascular mortality, all-cause mortality, and diabetes incidence after lifestyle intervention for people with impaired glucose tolerance in the Da Qing Diabetes Prevention Study: a 23-year follow-up study | 2          | Guangwei Li       | Peter H Bennett  | 2014    | CHN         | The Lancet Diabetes and Endocrinology | 808      | 73.45             | No      |
| Does diabetes prevention translate into reduced long-term vascular complications of diabetes?                                                                                                                     | 7          | David M. Nathan   | Neil H. White    | 2019    | USA         | Diabetologia                          | 85       | 14.17             | No      |
| The Cost-Effectiveness of Lifestyle Modification or Metformin in Preventing Type 2 Diabetes in Adults with Impaired Glucose Tolerance                                                                             | 2          | William H. Herman | Robert E. Ratner | 2005    | USA         | Annals of Internal Medicine           | 899      | 44.95             | No      |

Table S3.1 continued from previous page

| Title                                                                                                                                               | Study type | First author                                   | Last author                                    | Year | Nationality | Journal                                           | Cited by | Cited by per year | Sampled |
|-----------------------------------------------------------------------------------------------------------------------------------------------------|------------|------------------------------------------------|------------------------------------------------|------|-------------|---------------------------------------------------|----------|-------------------|---------|
| The 10-year cost-effectiveness of lifestyle intervention or metformin for diabetes prevention: an intent-to-treat analysis of the DPP/DPPOS         | 2          | The Diabetes Prevention Program Research Group | The Diabetes Prevention Program Research Group | 2012 | USA         | Diabetes Care                                     | 534      | 41.08             | No      |
| Impact of the YMCA of the USA Diabetes Prevention Program on Medicare spending and utilization                                                      | 4          | Maria Alva                                     | L. Lucia Rojas-Smith                           | 2017 | USA         | Health Affairs                                    | 57       | 7.13              | No      |
| Cost-effectiveness of diabetes prevention interventions targeting high-risk individuals and whole populations: a systematic review                  | 6          | Xilin Zhou                                     | Ping Zhang                                     | 2020 | USA         | Diabetes Care                                     | 151      | 30.2              | No      |
| Nutrition Therapy for Adults With Diabetes or Prediabetes: A Consensus Report                                                                       | 7          |                                                |                                                | 2019 | USA         | Diabetes Care                                     | 1418     | 236.33            | No      |
| Medical nutrition therapy and weight loss questions for the Evidence Analysis Library prevention of type 2 diabetes project: systematic reviews     | 6          | Hollie Raynor                                  | A. Lisa Moloney                                | 2017 | USA         | Journal of the Academy of Nutrition and Dietetics | 58       | 7.25              | No      |
| The effectiveness and cost of lifestyle interventions including nutrition education for diabetes prevention: a systematic review and meta-analysis. | 5          | Yu Sun                                         | Brenda Davy                                    | 2017 | USA         | Journal of the Academy of Nutrition and Dietetics | 239      | 29.88             | No      |
| Building therapeutic relationships: choosing words that put people first                                                                            | 7          | Jane Dickinson                                 | K. Melinda D. Maryniuk                         | 2017 | USA         | Clinical Diabetes                                 | 41       | 5.13              | No      |

Table S3.1 continued from previous page

| Title                                                                                                                                                                                                               | Study type | First author        | Last author         | Year | Nationality | Journal                                    | Cited by | Cited by per year | Sampled |
|---------------------------------------------------------------------------------------------------------------------------------------------------------------------------------------------------------------------|------------|---------------------|---------------------|------|-------------|--------------------------------------------|----------|-------------------|---------|
| Effect of weight loss with lifestyle intervention on risk of diabetes                                                                                                                                               | 2          | Richard F. Hamman   | Judith Wylie-Rosett | 2006 | USA         | Diabetes Care                              | 1706     | 89.79             | No      |
| Exercise Training, Without Weight Loss, Increases Insulin Sensitivity and Postheparin Plasma Lipase Activity in Previously Sedentary Adults                                                                         | 8          | Glen E. Duncan      | Peter W. Stacpoole  | 2003 | USA         | Diabetes Care                              | 649      | 29.5              | No      |
| Association of bariatric surgery with long-term remission of type 2 diabetes and with microvascular and macrovascular complications                                                                                 | 3          | Lars Sjöström       | Lena M. S. Carlsson | 2014 | SWE         | JAMA                                       | 1225     | 111.36            | No      |
| Dapagliflozin's Effects on Glycemia and Cardiovascular Risk Factors in High-Risk Patients With Type 2 Diabetes: A 24-Week, Multicenter, Randomized, Double-Blind, Placebo-Controlled Study With a 28-Week Extension | 1          | William T. Cefalu   | Shamik J. Parikh    | 2015 | USA         | Diabetes Care                              | 188      | 18.8              | No      |
| Food groups and risk of all-cause mortality: a systematic review and meta-analysis of prospective studies                                                                                                           | 5          | Schwingshackl Lukas | Boeing Heiner       | 2017 | AUT         | The American Journal of Clinical Nutrition | 659      | 82.38             | No      |
| An Update on the Mediterranean, Vegetarian, and DASH Eating Patterns in People With Type 2 Diabetes                                                                                                                 | 7          | Gretchen Benson     | Joy Hayes           | 2020 | USA         | Diabetes Spectrum                          | 26       | 5.2               | No      |

Table S3.1 continued from previous page

| Title                                                                                                                                                                                            | Study type | First author          | Last author             | Year | Nationality | Journal                                  | Cited by | Cited by per year | Sampled |
|--------------------------------------------------------------------------------------------------------------------------------------------------------------------------------------------------|------------|-----------------------|-------------------------|------|-------------|------------------------------------------|----------|-------------------|---------|
| Efficacy and safety of carbohydrate counting versus other forms of dietary advice in patients with type 1 diabetes mellitus: a systematic review and meta-analysis of randomised clinical trials | 5          | Carlos Builes-Montaño | E Natalia A Rojas-Henao | 2022 | COL         | Journal of Human Nutrition and Dietetics | 26       | 8.67              | No      |
| Simplifying carb counting: A randomized controlled study – Feasibility and efficacy of an individualized, simple, patient-centred carb counting tool                                             | 1          | Shulamit Witkow       | Rachel Golan            | 2023 | ISR         | Endocrinology, Diabetes & Metabolism     | 9        | 4.5               | No      |
| A Randomized Crossover Trial to Compare Automated Insulin Delivery (the Artificial Pancreas) With Carbohydrate Counting or Simplified Qualitative Meal-Size Estimation in Type 1 Diabetes        | 1          | Ahmad Haidar          | Rémi Rabasa-Lhoret      | 2023 | CAN         | Diabetes Care                            | 15       | 7.5               | No      |
| Prospective independent evaluation of the carbohydrate counting accuracy of two smartphone applications                                                                                          | 8          | Michael Joubert       | Yves Reznik             | 2021 | FRA         | Diabetes Therapy                         | 14       | 3.5               | No      |
| A Comparative Study on Carbohydrate Estimation: GoCARB vs. Dietitians                                                                                                                            | 8          | Maria F. Vasiloglou   | Zeno Stanga             | 2018 | CHE         | Nutrients                                | 86       | 12.29             | No      |
| The diabetes nutrition education study randomized controlled trial: A comparative effectiveness study of approaches to nutrition in diabetes self-management education                           | 1          | Michael E. Bowen      | Russell L. Rothman      | 2016 | USA         | Patient Education and Counseling         | 137      | 15.22             | No      |
| Defining food literacy: A scoping review                                                                                                                                                         | 7          | Emily Trueman         | Charlene Eliott         | 2017 | CAN         | Appetite                                 | 358      | 44.75             | No      |

Table S3.1 continued from previous page

| Title                                                                                                                                                                                                                                                                                                                    | Study type | First author         | Last author              | Year | Nationality | Journal                        | Cited by | Cited by per year | Sampled |
|--------------------------------------------------------------------------------------------------------------------------------------------------------------------------------------------------------------------------------------------------------------------------------------------------------------------------|------------|----------------------|--------------------------|------|-------------|--------------------------------|----------|-------------------|---------|
| Effectiveness of Early Time-Restricted Eating for Weight Loss, Fat Loss, and Cardiometabolic Health in Adults With Obesity                                                                                                                                                                                               | 1          | Humaira Jamshed      | Courtney M. Peterson     | 2022 | USA         | JAMA Internal Medicine         | 139      | 46.33             | No      |
| Effects of Time-Restricted Eating on Weight Loss and Other Metabolic Parameters in Women and Men With Overweight and Obesity                                                                                                                                                                                             | 1          | Dylan Lowe           | A. Ethan Weiss           | 2020 | USA         | JAMA Internal Medicine         | 474      | 94.8              | No      |
| Nutrition Therapy Recommendations for the Management of Adults With Diabetes                                                                                                                                                                                                                                             | 7          | Alison Evert         | B. William S. Yancy, Jr. | 2013 | USA         | Diabetes Care                  | 2202     | 183.5             | No      |
| Review of current evidence and clinical recommendations on the effects of low-carbohydrate and very-low-carbohydrate (including ketogenic) diets for the management of body weight and other cardiometabolic risk factors: A scientific statement from the National Lipid Association Nutrition and Lifestyle Task Force | 7          | Carol Kirkpatrick    | F. Kevin Maki            | 2019 | USA         | Journal of Clinical Lipidology | 378      | 63                | No      |
| Efficacy and safety of low and very low carbohydrate diets for type 2 diabetes remission: systematic review and meta-analysis of published and unpublished randomized trial data                                                                                                                                         | 5          | Joshua Z. Goldenberg | Bradley C. Johnston      | 2021 | USA         | BMJ                            | 362      | 90.5              | No      |

Table S3.1 continued from previous page

| Title                                                                                                                                                                                                                                                    | Study type | First author         | Last author        | Year | Nationality | Journal                                           | Cited by | Cited by per year | Sampled |
|----------------------------------------------------------------------------------------------------------------------------------------------------------------------------------------------------------------------------------------------------------|------------|----------------------|--------------------|------|-------------|---------------------------------------------------|----------|-------------------|---------|
| Carbohydrate restriction for diabetes: re-discovering centuries-old wisdom                                                                                                                                                                               | 7          | Belinda S. Lennerz   | David S. Ludwig    | 2021 | USA         | The Journal of Clinical Investigation             | 60       | 15                | No      |
| A network meta-analysis on the comparative efficacy of different dietary approaches on glycaemic control in patients with type 2 diabetes mellitus                                                                                                       | 6          | Lukas Schwing-shackl | Heiner Boe-ing     | 2018 | DEU         | European Journal of Epidemiology                  | 296      | 42.29             | No      |
| Academy of Nutrition and Dietetics Nutrition Practice Guideline for Type 1 and Type 2 Diabetes in Adults: Systematic Review of Evidence for Medical Nutrition Therapy Effectiveness and Recommendations for Integration into the Nutrition Care Process. | 6          | Marion Franz         | J Megan Robinson   | 2017 | USA         | Journal of the Academy of Nutrition and Dietetics | 380      | 47.5              | No      |
| Training in flexible, intensive insulin management to enable dietary freedom in people with type 1 diabetes: dose adjustment for normal eating (DAFNE) randomised controlled trial                                                                       | 1          | DAFNE Study Group    | DAFNE Study Group  | 2002 | GBR         | BMJ                                               | 1180     | 51.3              | No      |
| Diabetes Interactive Diary: A New Telemedicine System Enabling Flexible Diet and Insulin Therapy While Improving Quality of Life: An open-label, international, multicenter, randomized study                                                            | 1          | Maria C.E. Rossi     | Giacomo Vespasiani | 2010 | ITA         | Diabetes Care                                     | 232      | 15.47             | No      |

Table S3.1 continued from previous page

| Title                                                                                                                                                                                             | Study type | First author         | Last author        | Year   | Nationality | Journal                                           | Cited by | Cited by per year | Sampled |
|---------------------------------------------------------------------------------------------------------------------------------------------------------------------------------------------------|------------|----------------------|--------------------|--------|-------------|---------------------------------------------------|----------|-------------------|---------|
| Glycaemic control and severe hypoglycaemia following training in flexible, intensive insulin therapy to enable dietary freedom in people with type 1 diabetes: a prospective implementation study | 8          | A. Sämann            | U. A. Müller       | 2005   | DEU         | Diabetologia                                      | 267      | 13.35             | No      |
| Non?nutritive sweeteners for diabetes mellitus                                                                                                                                                    | 5          | Szimonetta Lohner    | Joerg Meerpohl     | J 2020 | HUN         | Cochrane Database of Systematic reviews           | 87       | 17.4              | No      |
| 2019 ACC/AHA Guideline on the Primary Prevention of Cardiovascular Disease: A Report of the American College of Cardiology/American Heart Association Task Force on Clinical Practice Guidelines  | 7          | Donna K. Arnett      | Boback Ziaean      | 2019   | USA         | Journal of the American College of Cardiology     | 6272     | 1045.33           | No      |
| Nutrition therapy for adults with diabetes or prediabetes: a consensus report                                                                                                                     | 7          | Alison B Evert       | William S Yancy Jr | 2019   | USA         | Diabetes Care                                     | 1413     | 235.5             | No      |
| Consumption of Beverages Containing Low-Calorie Sweeteners, Diet, and Cardiometabolic Health in Youth With Type 2 Diabetes                                                                        | 2          | Allison C. Sylvetsky | Laure El ghormli   | 2020   | USA         | Journal of the Academy of Nutrition and Dietetics | 10       | 2                 | No      |
| Exercise in adults with type 1 diabetes mellitus                                                                                                                                                  | 7          | Michael C. Riddell   | Anne L. Peters     | 2022   | CAN         | Nature Reviews Endocrinology                      | 51       | 17                | No      |

Table S3.1 continued from previous page

| Title                                                                                                                                                                                           | Study type | First author                  | Last author               | Year | Nationality | Journal                                 | Cited by | Cited by per year | Sampled |
|-------------------------------------------------------------------------------------------------------------------------------------------------------------------------------------------------|------------|-------------------------------|---------------------------|------|-------------|-----------------------------------------|----------|-------------------|---------|
| Lifestyle Interventions for Patients With and at Risk for Type 2 Diabetes: A Systematic Review and Meta-analysis                                                                                | 5          | Elizabeth Sumamo Schellenberg | Christina Korownyk        | 2013 | CAN         | Annals of Internal Medicine             | 699      | 58.25             | No      |
| Evidence-based behavioral interventions to promote diabetes management in children, adolescents, and families.                                                                                  | 7          | Hilliard, Marisa E            | Anderson, Barbara J.      | 2016 | USA         | American Psychologist                   | 176      | 19.56             | No      |
| Effective strategies for encouraging behavior change in people with diabetes                                                                                                                    | 7          | Korey Hood                    | K Carolyn E Ievers-Landis | 2015 | USA         | Diabetes Management                     | 125      | 12.5              | No      |
| Effect of group cognitive behavioural therapy on psychological stress and blood glucose in people with type 2 diabetes mellitus: A community-based cluster randomized controlled trial in China | 1          | Chunrong Xu                   | Peian Lou                 | 2020 | CHN         | Diabetic Medicine                       | 28       | 5.6               | No      |
| Cognitive behavioral therapy in adolescents with type 1 diabetes: an integrative review                                                                                                         | 6          | Kaitlyn Rechenberg            | Rebecca Koerner           | 2021 | USA         | Journal of Pediatric Nursing            | 35       | 8.75              | No      |
| The efficacy of cognitive behavioral therapy-based intervention on patients with diabetes: A meta-analysis                                                                                      | 5          | Yanni Li                      | Jing Sun                  | 2022 | AUS         | Diabetes Research and Clinical Practice | 25       | 8.33              | No      |

Table S3.1 continued from previous page

| Title                                                                                                                                                                                                | Study type | First author         | Last author         | Year | Nationality | Journal                                          | Cited by | Cited by per year | Sampled |
|------------------------------------------------------------------------------------------------------------------------------------------------------------------------------------------------------|------------|----------------------|---------------------|------|-------------|--------------------------------------------------|----------|-------------------|---------|
| Effectiveness of cognitive behavioral therapy-based interventions on psychological symptoms in adults with type 2 diabetes mellitus: An update review of randomized controlled trials                | 6          | Eugenia Vlachou      | Omar Cauli          | 2022 | GRC         | Journal of Diabetes and its Complications        | 33       | 11                | No      |
| Effect of a mindfulness programme for long-term care residents with type 2 diabetes: A cluster randomised controlled trial measuring outcomes of glycaemic control, relocation stress and depression | 1          | Shu-Ming Chen        | Chiung-Jung (Jo) Wu | 2020 | TWN         | International Journal of Older People Nursing    | 29       | 5.8               | No      |
| Evaluation of the Effects of 12 Weeks Mindfulness-Based Stress Reduction on Glycemic Control and Mental Health Indices in Women with Diabetes Mellitus Type 2                                        | 1          | Nikkhah Ravari, Omid | Babak, Anahita      | 2020 | IRA         | Advanced Biomedical Research                     | 23       | 4.6               | No      |
| Virtual group appointments reduce distress and improve care management in young adults with type 1 diabetes                                                                                          | 1          | Daniel I. Bisno      | Jennifer K. Raymond | 2022 | USA         | Journal of Diabetes Science and Technology       | 42       | 14                | No      |
| Effective interventions for reducing diabetes distress: systematic review and meta-analysis                                                                                                          | 5          | Jackie Sturt         | Lawrence Fisher     | 2015 | GBR         | International Diabetes Nursing                   | 164      | 16.4              | No      |
| 2022 National standards for diabetes self-management education and support                                                                                                                           | 7          | Jody Davis           | Suzanne Villalobos  | 2022 | USA         | The Science of Diabetes Self-Management and Care | 226      | 75.33             | No      |

Table S3.1 continued from previous page

| Title                                                                                                                                                                        | Study type | First author            | Last author           | Year | Nationality | Journal                                    | Cited by | Cited by per year | Sampled |
|------------------------------------------------------------------------------------------------------------------------------------------------------------------------------|------------|-------------------------|-----------------------|------|-------------|--------------------------------------------|----------|-------------------|---------|
| Depression in Adults With Diabetes: Results of 5-yr Follow-Up Study                                                                                                          | 3          | Patrick J. Lustman      | Ray E. Clouse         | 1988 | USA         | Diabetes Care                              | 393      | 10.62             | No      |
| Elevated Depression Symptoms, Antidepressant Medicine Use, and Risk of Developing Diabetes During the Diabetes Prevention Program                                            | 2          | Richard R. Rubin        | William C. Knowler    | 2008 | USA         | Diabetes Care                              | 319      | 18.76             | No      |
| Effectiveness of Internet and Phone-Based Interventions on Diabetes Management of Children and Adolescents With Type 1 Diabetes: A Systematic Review                         | 5          | Xiaolei Zhao            | Silin Zheng           | 2021 | CHN         | Worldviews on Evidence-based Nursing       | 10       | 2.5               | No      |
| Internet Delivered Diabetes Self-Management Education: A Review                                                                                                              | 6          | Katherine Pereira       | Allison Vorderstrasse | 2015 | USA         | Diabetes Technology & Therapeutics         | 162      | 16.2              | No      |
| Long-Term Outcomes of a Web-Based Diabetes Prevention Program: 2-Year Results of a Single-Arm Longitudinal Study                                                             | 8          | S. Cameron Sepah        | Anne L. Peters        | 2015 | USA         | Journal of Medical Internet Research       | 232      | 23.2              | No      |
| A Systematic Review of Reviews Evaluating Technology-Enabled Diabetes Self-Management Education and Support                                                                  | 6          | Deborah A. Greenwood    | Malinda Peebles       | 2017 | USA         | Journal of Diabetes Science and Technology | 553      | 69.13             | No      |
| Long-Term Effects of a Novel Continuous Remote Care Intervention Including Nutritional Ketosis for the Management of Type 2 Diabetes: A 2-Year Non-randomized Clinical Trial | 8          | Shaminie J. Athinayanan | James P. McCarter     | 2019 | USA         | Frontiers in Endocrinology                 | 342      | 57                | No      |

Table S3.1 continued from previous page

| Title                                                                                                                                                             | Study type | First author       | Last author         | Year | Nationality | Journal                                         | Cited by | Cited by per year | Sampled |
|-------------------------------------------------------------------------------------------------------------------------------------------------------------------|------------|--------------------|---------------------|------|-------------|-------------------------------------------------|----------|-------------------|---------|
| Effectiveness and Safety of a Novel Care Model for the Management of Type 2 Diabetes at 1 Year: An Open-Label, Non-Randomized, Controlled Study                   | 8          | Sarah J. Hallberg  | Jeff S. Volek       | 2018 | USA         | Diabetes Therapy                                | 473      | 67.57             | No      |
| Telemedicine in the Management of Type 1 Diabetes                                                                                                                 | 8          | Timothy Xu         | Mary Rhee           | 2018 | USA         | CDC Preventing Chronic Disease                  | 161      | 23                | No      |
| Web-based interventions for dietary behavior in adults with type 2 diabetes: systematic review of randomized controlled trials                                    | 6          | Jedha Dening       | Ralph Madison       | 2020 | AUS         | Journal of Medical Internet Research            | 47       | 9.4               | No      |
| Telehealth Interventions to Improve Diabetes Management Among Black and Hispanic Patients: a Systematic Review and Meta-Analysis                                  | 5          | Andrew Anderson    | Rishab Chimmanamada | 2022 | USA         | Journal of Racial and Ethnic Health Disparities | 50       | 16.67             | No      |
| Effect of Diabetes Health Coaching on Glycemic Control and Quality of Life in Adults Living With Type 2 Diabetes: A Community-Based, Randomized, Controlled Trial | 1          | Diana Sherifali    | Hertzel C. Gerstein | 2021 | CAN         | Canadian Journal of Diabetes                    | 27       | 6.75              | No      |
| Telemedicine-Assisted Self-Management Program for Type 2 Diabetes Patients                                                                                        | 1          | Katja von Storch   | Christiane Woopen   | 2019 | DEU         | Diabetes Technology & Therapeutics              | 113      | 18.83             | No      |
| Night-shift work is associated with poorer glycaemic control in patients with type 2 diabetes                                                                     | 3          | Areesa Manodpitong | Sirimon Reutrakul   | 2017 | THA         | Journal of Sleep Research                       | 93       | 11.63             | No      |

Table S3.1 continued from previous page

| Title                                                                                                                                                                                                 | Study type | First author                  | Last author                   | Year | Nationality | Journal                                                          | Cited by | Cited by per year | Sampled |
|-------------------------------------------------------------------------------------------------------------------------------------------------------------------------------------------------------|------------|-------------------------------|-------------------------------|------|-------------|------------------------------------------------------------------|----------|-------------------|---------|
| Very-Low-Calorie Diets and Sustained Weight Loss                                                                                                                                                      | 7          | Wim H.M. Saris                | Wim H.M. Saris                | 2012 | NLD         | Obesity Research                                                 | 348      | 26.77             | No      |
| Micronutrient quality of weight-loss diets that focus on macronutrients: results from the A TO Z study                                                                                                | 1          | Gardner Christopher D         | Cherin Rise                   | 2010 | USA         | The American Journal of Clinical Nutrition                       | 132      | 8.8               | No      |
| Effects of anti-obesity drugs, diet, and exercise on weight-loss maintenance after a very-low-calorie diet or low-calorie diet: a systematic review and meta-analysis of randomized controlled trials | 5          | Kari Johansson                | Erik Hemmingsson              | 2014 | SWE         | The American Journal of Clinical Nutrition                       | 338      | 30.73             | No      |
| UK prospective diabetes study 7: Response of fasting plasma glucose to diet therapy in newly presenting type II diabetic patients                                                                     | 1          | UKPDS group                   | UKPDS group                   | 1990 | GBR         | Metabolism                                                       | 123      | 3.51              | No      |
| Beneficial health effects of modest weight loss                                                                                                                                                       | 7          | Goldstein DJ                  | Goldstein DJ                  | 1992 | USA         | International Journal of Obesity and Related Metabolic Disorders | 2066     | 62.61             | No      |
| The Evidence for the Effectiveness of Medical Nutrition Therapy in Diabetes Management                                                                                                                | 7          | Joyce Green Pastors           | Karmeen Kulkarni              | 2002 | USA         | Diabetes Care                                                    | 728      | 31.65             | No      |
| Cardiovascular Effects of Intensive Lifestyle Intervention in Type 2 Diabetes                                                                                                                         | 1          | The Look AHEAD Research Group | The Look AHEAD Research Group | 2013 | USA         | The NEJM                                                         | 3139     | 261.58            | No      |

Table S3.1 continued from previous page

| Title                                                                                                                                                                                        | Study type | First author                  | Last author                   | Year | Nationality | Journal                                           | Cited by | Cited by per year | Sampled |
|----------------------------------------------------------------------------------------------------------------------------------------------------------------------------------------------|------------|-------------------------------|-------------------------------|------|-------------|---------------------------------------------------|----------|-------------------|---------|
| Eight-year weight losses with an intensive lifestyle intervention: The look AHEAD study                                                                                                      | 1          | The Look AHEAD Research Group | The Look AHEAD Research Group | 2013 | USA         | Obesity                                           | 851      | 70.92             | No      |
| Lifestyle Weight-Loss Intervention Outcomes in Overweight and Obese Adults with Type 2 Diabetes: A Systematic Review and Meta-Analysis of Randomized Clinical Trials                         | 5          | Marion Franz                  | J. Jeffrey VanWormer          | 2015 | USA         | Journal of the Academy of Nutrition and Dietetics | 786      | 78.6              | No      |
| Long-term effects of intensive multifactorial therapy in individuals with screen-detected type 2 diabetes in primary care: 10-year follow-up of the ADDITION-Europe cluster-randomised trial | 1          | Simon Griffin                 | J. Anelli Sandbæk             | 2019 | GBR         | The Lancet Diabetes & Endocrinology               | 51       | 8.5               | No      |
| Treatment intensification with stepwise addition of prandial insulin aspart boluses compared with full basal-bolus therapy (FullSTEP Study): a randomised, treat-to-target clinical trial    | 1          | Helena W Rodbard              | David HW Shu                  | 2014 | USA         | The Lancet Diabetes & Endocrinology               | 122      | 11.09             | No      |
| Salt Reduction to Prevent Hypertension and Cardiovascular Disease: JACC State-of-the-Art Review                                                                                              | 7          | Feng J. He                    | Graham A. MacGregor           | 2020 | GBR         | Journal of the American College of Cardiology     | 530      | 106               | No      |

Table S3.1 continued from previous page

| Title                                                                                                                           | Study type | First author     | Last author               | Year | Nationality | Journal                                                             | Cited by | Cited by per year | Sampled |
|---------------------------------------------------------------------------------------------------------------------------------|------------|------------------|---------------------------|------|-------------|---------------------------------------------------------------------|----------|-------------------|---------|
| Physical activity, all-cause and cardiovascular mortality, and cardiovascular disease                                           | 6          | William E Kraus  | Katrina L Piercy          | 2019 | USA         | Medicine and science in sports and exercise                         | 584      | 97.33             | No      |
| Behaviour change techniques targeting both diet and physical activity in type 2 diabetes: A systematic review and meta-analysis | 5          | Kevin A. Cradock | Kathleen A. Martin Ginnis | 2017 | IRE         | International Journal of Behavioral Nutrition and Physical Activity | 383      | 47.88             | No      |
| Investigating weight loss in the elderly                                                                                        | 7          | GEORGE SZONYI    | GEORGE SZONYI             | 2005 | ZAF         | Modern Medicine of South Africa                                     | 0        | 0                 | No      |

## **File S4**

### **Causal linking words in guidelines and original studies**

Table S4.1: Causal linking word frequencies

| Guideline statement ( $n = 114$ ) |            |              | OS abstract ( $n = 81$ ) |            |              | OS main text ( $n = 183$ ) |            |              |
|-----------------------------------|------------|--------------|--------------------------|------------|--------------|----------------------------|------------|--------------|
| Word                              | Wtd. Freq. | Unwtd. Freq. | Word                     | Wtd. Freq. | Unwtd. Freq. | Word                       | Wtd. Freq. | Unwtd. Freq. |
| benefit                           | 14.3%      | 11.9%        | associated               | 24.1%      | 21.1%        | associated                 | 17.5%      | 16.7%        |
| reduce                            | 12.5%      | 12.5%        | reduce                   | 15.4%      | 14.7%        | effect                     | 14.2%      | 13.1%        |
| improve                           | 11.7%      | 11.3%        | effect                   | 11.7%      | 10.5%        | improve                    | 13.0%      | 13.1%        |
| associated                        | 10.8%      | 9.52%        | improve                  | 7.82%      | 8.42%        | reduce                     | 10.3%      | 10.1%        |
| effect                            | 7.23%      | 5.95%        | benefit                  | 4.94%      | 4.21%        | benefit                    | 6.19%      | 7.07%        |
| increase                          | 6.29%      | 6.55%        | lower                    | 4.53%      | 5.26%        | lower                      | 3.01%      | 3.03%        |
| maintain                          | 2.19%      | 1.79%        | greater                  | 2.47%      | 3.16%        | increase                   | 2.73%      | 3.54%        |
| help                              | 2.05%      | 2.98%        | promise                  | 2.47%      | 2.11%        | difference                 | 2.73%      | 2.53%        |
|                                   |            |              | result in                |            |              |                            |            |              |
| decrease                          | 1.61%      | 1.79%        | achieve                  | 1.85%      | 2.11%        | causal                     | 2.19%      | 2.02%        |
|                                   |            |              | decrease                 |            |              | cost effective             |            |              |
|                                   |            |              |                          |            |              | greater                    |            |              |
| risk                              | 1.32%      | 1.79%        | increase                 | 1.65%      | 3.16%        | lead                       | 1.64%      | 2.02%        |
| greater                           | 1.32%      | 1.19%        | better                   | 1.65%      | 2.11%        | help                       | 1.64%      | 1.52%        |
| link to                           |            |              |                          |            |              | promise                    |            |              |
| result in                         |            |              |                          |            |              | result in                  |            |              |

Table S4.1 (Continued)

| Guideline statement |            |              | OS abstract |            |              | OS main text |            |              |
|---------------------|------------|--------------|-------------|------------|--------------|--------------|------------|--------------|
| Word                | Wtd. Freq. | Unwtd. Freq. | Word        | Wtd. Freq. | Unwtd. Freq. | Word         | Wtd. Freq. | Unwtd. Freq. |
| contribute to       | 1.17%      | 1.19%        | ameliorate  | 1.23%      | 1.05%        | better       | 1.09%      | 1.01%        |
|                     |            |              | consequence |            |              | inferior     |            |              |
|                     |            |              | contribute  |            |              | superior     |            |              |
|                     |            |              | difference  |            |              | useful       |            |              |
|                     |            |              | gain        |            |              |              |            |              |
|                     |            |              | higher      |            |              |              |            |              |
|                     |            |              | impact      |            |              |              |            |              |
|                     |            |              | more        |            |              |              |            |              |
|                     |            |              | significant |            |              |              |            |              |
|                     |            |              | similar     |            |              |              |            |              |
|                     |            |              | superior    |            |              |              |            |              |

OS, original study; Wtd., weighted; Freq., frequency; Unwtd., unweighted. The weighted and unweighted frequencies take the total number of occurrence of all causal linking words as denominator. For weighted frequency, each occurrence of word is weighted by the reciprocal of total numbers of causal linking words in the associated sentence. Words of same weighted and unweighted rankings are shown in one row. Word list is truncated at weighted frequency of 1.00% because there are too many ties to display with frequencies less than 1.00%. Confidence intervals and inference statistics for between-group comparison are not displayed, as the contents in this table serve for pure descriptive purpose.



## References cited in supplementary files

1. American Diabetes Association Professional Practice Committee, ElSayed NA, Aleppo G, et al. 3. Prevention or Delay of Diabetes and Associated Comorbidities: Standards of Care in Diabetes—2024. *Diabetes Care* 2024;47:S43–S51.
2. American Diabetes Association Professional Practice Committee, ElSayed NA, Aleppo G, et al. 5. Facilitating Positive Health Behaviors and Well-being to Improve Health Outcomes: Standards of Care in Diabetes—2024. *Diabetes Care* 2024;47:S77–S110.
3. American Diabetes Association Professional Practice Committee, ElSayed NA, Aleppo G, et al. 8. Obesity and Weight Management for the Prevention and Treatment of Type 2 Diabetes: Standards of Care in Diabetes—2024. *Diabetes Care* 2024;47:S145–S157.
4. American Diabetes Association Professional Practice Committee, ElSayed NA, Aleppo G, et al. 10. Cardiovascular Disease and Risk Management: Standards of Care in Diabetes—2024. *Diabetes Care* 2024;47:S179–S218.
5. American Diabetes Association Professional Practice Committee, ElSayed NA, Aleppo G, et al. 13. Older Adults: Standards of Care in Diabetes—2024. *Diabetes Care* 2024;47:S244–S257.
6. Marx N, Federici M, Schütt K, et al. 2023 ESC Guidelines for the management of cardiovascular disease in patients with diabetes: Developed by the task force on the management of cardiovascular disease in patients with diabetes of the European Society of Cardiology (ESC). *European Heart Journal* 2023;44:4043–140.
7. Haber NA, Wieten SE, Rohrer JM, et al. Causal and Associational Language in Observational Health Research: A Systematic Evaluation. *American Journal of Epidemiology* 2022;191:2084–97.
8. Smit JM, Krijthe JH, Kant WMR, et al. Causal inference using observational intensive care unit data: a scoping review and recommendations for future practice. *npj Digital Medicine* 2023;6:1–11.
